# Supplementary material for: IRENE: a fluId layeR finitE-elemeNt softwarE
Source: arXiv:2506.17827 source file (2026-10-19)
Supplement: Supplementary file 1 [file supplementary.pdf]

# Supplementary material for:

# irene

# A fluid layer finite-element software

Dennis Wörthmüller[1,2], Gaetano Ferraro[1,2,3], Pierre Sens[1,2], and Michele Castellana*[1,2]

[1]Institut Curie, PSL Research University, Paris, France
[2]CNRS UMR168, 11 rue Pierre et Marie Curie, 75005, Paris,France
[2]Polytechnic University of Turin, Corso Castelfidardo 39, 10129 Turin, Italy

## S1 Differential-geometric definitions

In this Section, we will shortly report some basic differential-geometric definitions used in irene; details can be found, for instance, in [1, 2, 3]. These definitions are implemented in irene's `geometry` module.

In irene, we will consider two-dimensional manifolds $\mathscr{M}$ embedded in three-dimensional Euclidean space $\mathbb{R}^3$, where $\mathscr{M}$ is described by two coordinates $x^1, x^2$ through the parameterization [4, 5]

$$\boldsymbol{X}(x^1, x^2), \tag{S1}$$

and $\boldsymbol{X}$ is a vector in $\mathbb{R}^3$. We will use Einstein notation for indexes $i, j, \cdots$, which we will use to denote forms, vectors and tensors. Other coordinates which we will adopt in this manuscript are radial coordinates $x^1 = r, x^2 = \theta$ in the $xy$ plane.

### S1.1 Fundamental scalars and tensors

The tangent vectors to the coordinate lines, the normal to $\mathscr{M}$, which we denote by $\hat{N}$, the metric tensor $g$ and the second fundamental form $b$ are, respectively,

$$\mathbf{e}_i = \partial_i \boldsymbol{X}, \tag{S2}$$

$$\hat{N} = \frac{\mathbf{e}_1 \times \mathbf{e}_2}{|\mathbf{e}_1 \times \mathbf{e}_2|}, \tag{S3}$$

$$g_{ij} = \mathbf{e}_i \cdot \mathbf{e}_j, \tag{S4}$$

$$b_{ij} = \hat{N} \cdot \partial_i \mathbf{e}_j. \tag{S5}$$

The mean and gaussian curvatures are, respectively,

$$H = \frac{1}{2} b^i_i \tag{S6}$$

$$K = |b|/|g|, \tag{S7}$$

where $||$ denotes the determinant, and indexes are raised and lowered with $g$.

*Corresponding author: michele.castellana@curie.fr

## S1.2 Covariant derivative

The covariant derivative of a $n$-contravariant and $m$-covariant tensor $T^{i_1 \cdots i_n}_{j_1 \cdots j_m}$ is given by

$$\begin{aligned}\nabla_i T^{i_1 \cdots i_n}_{j_1 \cdots j_m} =& \partial_i T^{i_1 \cdots i_n}_{j_1 \cdots j_m} \\ &+ \Gamma^{i_1}_{ki} T^{k\, i_2 \cdots\, i_n}_{j_1 \cdots j_m} + \cdots + \Gamma^{i_p}_{ki} T^{i_1 \cdots i_{p-1}\, k\, i_{p+1} \cdots\, i_n}_{j_1 \cdots j_m} + \cdots \Gamma^{i_n}_{ki} T^{i_1 \cdots\, i_{n-1}\, k}_{j_1 - \cdots j_m} \\ &- \Gamma^{k}_{j_1 i} T^{i_1 \cdots i_n}_{k\, j_2 \cdots j_m} \cdots - \Gamma^{k}_{j_p i} T^{i_1 \cdots i_n}_{j_1 \cdots j_{p-1}\, i\, j_{p+1} \cdots j_m} - \cdots - \Gamma^{k}_{j_m i} T^{i_1 \cdots i_n}_{j_1 \cdots j_{m-1}\, k}.\end{aligned} \tag{S8}$$

where

$$\Gamma^i_{jk} \equiv \frac{1}{2} g^{il} \left( \partial_j g_{lk} + \partial_k g_{lj} - \partial_l g_{jk} \right), \tag{S9}$$

are the Christoffel symbols of the second kind.

## S1.3 Laplace-Beltrami operator

The Laplace-Beltrami operator [6] $\nabla_{\text{LB}}$ applied to a scalar $f$ and a vector $v$ reads, respectively,

$$\nabla_{\text{LB}} f = - \frac{1}{\sqrt{|g|}} \partial_i \left( \sqrt{|g|} g^{ij} \partial_j f \right), \tag{S10}$$

$$\nabla_{\text{LB}} v^i = - \sqrt{|g|} g^{il} g^{jk} \epsilon_{jl} \partial_k \left[ \sqrt{|g|} g^{mn} g^{op} \epsilon_{mo} \partial_n \left( g_{pq} v^q \right) \right], \tag{S11}$$

where $\epsilon_{ij}$ is the Levi-Civita antisymmetric symbol [1].

The Laplace-Beltrami operator is related to the covariant derivative by [6]

$$\nabla_{\text{LB}} \mu = -\nabla_i \nabla^i \mu. \tag{S12}$$

## S1.4 Curves

Let us consider a curve $\gamma$ in $\mathscr{M}$, parametrized with curvilinear coordinate $s$; the points of $\gamma$ have coordinates $x^i(s)$. We will denote by $\mathfrak{n}$ the vector normal to $\gamma$, where $\mathfrak{n}$ belongs to the tangent bundle of $\mathscr{M}$ [1].

## S1.5 Pull-back of the metric

Given a curve $\gamma$ in $\mathscr{M}$, the natural mapping which associates to every point of $\gamma$ the same point considered as part of $\mathscr{M}$, see Fig. 1, yields a mapping $s \longrightarrow x^i(s)$. The pull-back of $g$ on $\gamma$ is then

$$h = \frac{dx^i}{ds} \frac{dx^j}{ds} g_{ij}. \tag{S13}$$

In particular, this definition applies to the case where $\gamma$ is a boundary of $\mathscr{M}$, see Fig. 1. In what follows, we will provide two examples of pull-backs of the metric on specific boundaries.

### S1.5.1 Pull-back on a rectangular edge

Consider the lower edge $\partial\Omega_{\sqsubset}$ in Fig. 1, parameterized with the coordinate $s = x$, where $0 \le x \le L$ is the abscissa in the $x^1 x^2$ plane. Then

$$\begin{aligned} x^1(s) =& s, \\ x^2(s) =& 0, \end{aligned} \tag{S14}$$

and $h$ is given by Eqs. (S13) and (S14).

### S1.5.2 Pull-back on a circle

Consider a circular boundary $\partial\Omega_{\circ}$ given by a circle of radius $r$ centered at $c_r$, see Fig. 1. We parameterize $\mathscr{M}$ with Cartesian coordinates and $\partial\Omega_{\circ}$ with the coordinate $s = \theta$, where $0 \leq \theta < 2\pi$ is the angle of polar coordinates in the $x^1x^2$ plane centered at $c_r$, see Section S1.7. Then

$$\begin{aligned} x^1(s) &= c_r^1 + r\cos s, \\ x^2(s) &= c_r^2 + r\sin s, \end{aligned} \tag{S15}$$

and $h$ is given by Eqs. (S13) and (S15).

## S1.6 Integration measures

We will denote the integral of a quantity over $\Omega$ by

$$\langle\cdot\rangle_\Omega = \int_\Omega \sqrt{|g|}\mathrm{d}x^1\mathrm{d}x^2 \,\cdot, \tag{S16}$$

and the integral over a boundary $\partial\Omega$ by

$$\langle\cdot\rangle_{\partial\Omega} = \int_{\partial\Omega} \mathrm{d}s\sqrt{|h|}\,\cdot, \tag{S17}$$

where $h$ is the pull-back of $g$ on $\partial\Omega$, see Section S1.5. The quantity $\mathrm{d}s\sqrt{h}$ has the geometrical meaning of the length of the line element $\mathrm{d}s$ of $\partial\Omega$ with respect to the Euclidean metric in $\mathbb{R}^3$.

The following identity for integration by parts [7] will be used repeatedly:

$$\left\langle U\nabla_i V^i\right\rangle_\Omega = -\left\langle V^i\nabla_i U\right\rangle_\Omega + \left\langle UV^i n_i\right\rangle_{\partial\Omega}, \tag{S18}$$

$$\left\langle T^{ij}\nabla_i W_j\right\rangle_\Omega = -\left\langle W_j\nabla_i T^{ij}\right\rangle_\Omega + \left\langle n_i T^{ij} W_j\right\rangle_{\partial\Omega}, \tag{S19}$$

where $U$, $V$, $W$ and $T$ are a scalar, a vector, a one-form and two-contravariant tensor, respectively. Also, $n$ is a vector field in the tangent bundle of $\mathscr{M}$ normal to $\partial\Omega$ and directed outside $\mathscr{M}$, see Fig. 1, and normalized to unity:

$$n^i n_i = 1. \tag{S20}$$

## S1.7 Coordinates

One possible coordinate choice is given by the Monge parameterization [8, 3], where $x^1 = x$ and $x^2 = y$ are the coordinates in the Cartesian $\mathbb{R}^2$ plane, see Fig. 1. In this parametrization, Eq. (S1) reads $X^1 = x$, $X^2 = y$ and $X^3 = z(x, y)$, and the tangent vectors to $\mathscr{M}$, Eq. (S2), are

$$\begin{aligned} \mathbf{e}_1 &= (1, 0, \partial_1 z), \\ \mathbf{e}_2 &= (0, 1, \partial_2 z). \end{aligned} \tag{S21}$$

For radially symmetric variational problems (VPs), see for example Figs. S1 to S3, we will use radial coordinates, i.e., $x^1 = r$, $x^2 = \theta$.

## S1.8 Geometries

In what follows, we will discuss the types of geometries considered in irene.

1. **Ring.** $\mathscr{M}$ is defined on a ring on the $\mathbb{R}^2$ plane, with radii $r$ and $R$ and delimited by two concentric circles centered at the origin.

2. **Rectangle.**

   $\mathscr{M}$ is defined on a rectangle on the $\mathbb{R}^2$ plane with sizes $L$ and $h$, and whose bottom-left vertex coincides with the origin.

3. **Rectangle with circular hole.**

   $\mathscr{M}$ is defined on the rectangle of Case 2, with a circular hole centered at $\mathbf{c}$ and with radius $r$, see Fig. 1.

# S2 Forces

In order to obtain the forces exerted on an element of $\partial\Omega$ or on an element of $\partial\Omega$, we introduce the rate-of-deformation tensor [9, 5]

$$d_{ij} \equiv \frac{1}{2}\left(\nabla_i v_j + \nabla_j v_i\right) - w b_{ij}, \tag{S22}$$

and the momentum-flux tensor [10]

$$\Pi_{ij} \equiv -\sigma g_{ij} - 2\eta\, d_{ij}. \tag{S23}$$

The tangential and normal viscous force exerted by the fluid on a fluid element [6] are, respectively,

$$f_\eta{}^i \equiv 2\eta \nabla_j d^{ij} \tag{S24}$$

$$= \eta\left[-\nabla_{\mathrm{LB}} v^i - 2\left(b^{ij} - 2\,H\, g^{ij}\nabla_j w\right) + 2K v^i\right], \tag{S25}$$

$$\mathfrak{f}_\eta \equiv 2\eta\left[(\nabla^i v^j) b_{ij} - 2w(2H^2 - K)\right]. \tag{S26}$$

The elastic force exerted by the fluid on a fluid element, and directed along the normal $\hat{N}$ of $\mathscr{M}$, is [6]

$$f_\kappa \equiv 2\kappa\left[\nabla_{\mathrm{LB}} H - 2H(H^2 - K)\right]. \tag{S27}$$

The force, due to surface tension and viscosity, exerted on an element $\mathrm{d}s$ of a curve $\gamma \in \mathscr{M}$, see Section S1.4, reads

$$\mathrm{d}F^i = \Pi^{ij}\mathfrak{n}_j\sqrt{|h|}\mathrm{d}s, \tag{S28}$$

where $\mathfrak{n}$ and $h$ are defined in Sections S1.4 and S1.5, respectively.

# S3 Variational formulations

## S3.1 Steady state

### S3.1.1 Steady state with no flows

By multiplying Eq. (16) by $\sqrt{|g|}$ and by the test functions $\nu_z$, $\nu_\omega{}^i$ and $\nu_\mu$ for the fields, $z$, $\omega_i$ and $\mu$, respectively, and by taking the average (S16), we obtain

$$\left\langle \left\{\kappa\left[\nabla_{\mathrm{LB}}\mu - 2\mu(\mu^2 - K)\right] + \sigma\mu\right\}\nu_z \right\rangle_\Omega = 0, \tag{S29}$$

$$\left\langle (\omega_i - \nabla_i z)\nu_\omega{}^i \right\rangle_\Omega = 0, \tag{S30}$$

$$F_\mu = 0, \tag{S31}$$

where

$$F_\mu \equiv \left\langle [\mu - H(\omega)]\nu_\mu \right\rangle_\Omega + G_\mu, \tag{S32}$$

and

$$G_\mu \equiv \frac{\alpha}{l}\left\langle [\mu - H(\omega)]\nu_\mu \right\rangle_{\partial\Omega}. \tag{S33}$$

Here, $G_\mu$ is a penalty term used to enforce Eq. (15) on $\partial\Omega$, $\alpha$ is a constant coefficient and $l$ the smallest cell diameter across all cells in the mesh [11]. Throughout our analysis, we will chose the constant $\alpha$ relative to penalty terms large enough in such a way that the boundary condition (BC) enforced by the penalty term is satisfied [12, 13].

We observe that, in the VP above, the test functions of scalar fields, e.g., $z$ and $\mu$, are scalars, and the test function of the one form $\omega$, $\nu_\omega$, is a vector. As a result, the mixed VP [14] given by Eqs. (S29) to (S31) preserves the covariance of Eq. (16).

As we discussed in Section 3.1.1, the presence of second derivatives in the term $\nabla_{\mathrm{LB}}\mu$ of Eq. (S29) would lead to an ill-posed VP. We will thus integrate by parts that term as follows

$$\begin{aligned}\left\langle (\nabla_{\mathrm{LB}}\mu)\nu_z\right\rangle_\Omega &= -\left\langle (\nabla_i\nabla^i\mu)\nu_z\right\rangle_\Omega\\ &= \left\langle (\nabla^i\mu)\nabla_i\nu_z\right\rangle_\Omega - \left\langle (\nabla^i\mu)n_i\nu_z\right\rangle_{\partial\Omega},\end{aligned} \tag{S34}$$

where in the first line we substituted Eq. (S12) and in the second we used Eq. (S18).

We now integrate by parts the second term in Eq. (S30). Given that Eq. (S30) involves a first derivative, such by-parts integration is not necessary because of the second-derivative issue discussed above. However, this integration by parts is convenient, because it will allow us to impose some BCs in weak form [15, 14], and thus to make 's weak form more portable with respect to different types of BCs. Proceeding along the same lines, in what follows we will perform other by-parts integrations because of such portability argument.

Proceeding along the same lines for the second term in Eq. (S30), we have

$$\left\langle (\nabla_i z) \nu_\omega{}^i \right\rangle_\Omega = - \left\langle z \, \nabla_i \nu_\omega{}^i \right\rangle_\Omega + \left\langle n_i \, z \, \nu_\omega{}^i \right\rangle_{\partial\Omega}, \tag{S35}$$

where we used Eq. (S18).

Combining Eqs. (S29) to (S31), (S34) and (S35), we obtain the functionals for the VP:

$$F_w \equiv \left\langle \kappa (\nabla^i \mu) \nabla_i \nu_z + \left[ -2\kappa\mu(\mu^2 - K) + \sigma\mu \right] \nu_z \right\rangle_\Omega - \kappa \left\langle (\nabla^i \mu) n_i \nu_z \right\rangle_{\partial\Omega}, \tag{S36}$$

$$F_\omega \equiv \left\langle \omega_i \nu_\omega{}^i + z \nabla_i \nu_\omega{}^i \right\rangle_\Omega - \left\langle n_i \, z \, \nu_\omega{}^i \right\rangle_{\partial\Omega}. \tag{S37}$$

This VP, whose BCs will be discussed in the following, is implemented in the `steady_state_no_flow` module.

In order to demonstrate 's flexibility as for the implementation of BCs, in what follows we will specify two sets of BCs for the VP. Here an in what follows, all BCs yield the same number of constraints for the partial differential equation (PDE) solution [16].

1. **Fixed-height boundary conditions.**

   (a) **Ring geometry.**

   For the ring geometry of Case 1 in Section S1.8, we consider the BCs

$$z = z_{\odot} \text{ on } \partial\Omega_{\odot}, \tag{S38}$$

$$z = z_{\bigcirc} \text{ on } \partial\Omega_{\bigcirc}, \tag{S39}$$

$$n^i \nabla_i z = \psi_{\odot} \text{ on } \partial\Omega_{\odot} \tag{S40}$$

$$n^i \nabla_i z = \psi_{\bigcirc} \text{ on } \partial\Omega_{\bigcirc}. \tag{S41}$$

   Equations (S38) and (S39) fix the height of the manifold at both the inner and outer circle, $\partial\Omega_{\odot}$ and $\partial\Omega_{\bigcirc}$, respectively, while Eqs. (S40) and (S41) fix the derivative of the manifold along the normal $n$ at both circles.

   The resulting boundary-value problem (BVP) is given by

$$F_w = 0, \tag{S42}$$

$$F_\omega = 0, \tag{S43}$$

$$F_\mu = 0, \tag{S44}$$

   in which the BCs (S38) and (S39) are enforced as Dirichlet BCs. In addition, Eqs. (S40) and (S41) are imposed by means of the penalty method [11], by adding to the VP the functional

$$G_\omega \equiv \frac{\alpha}{l} \left[ \langle (n^i \omega_i - \psi_{\odot}) n_j \nu_\omega{}^j \rangle_{\partial\Omega_{\odot}} + \langle (n^i \omega_i - \psi_{\bigcirc}) n_j \nu_\omega{}^j \rangle_{\partial\Omega_{\bigcirc}} \right], \tag{S45}$$

   in which we used the definition (14).

   This VP is solved in the `steady_state_no_flow` module as `variational_problem_bc_ring`, see Fig. S1.

(b) **Rectangle-with-circle geometry.**

For the geometry of Case 3 in Section S1.8, we consider the BCs

$$z = z_{\square} \text{ on } \partial\Omega_{\square}, \tag{S46}$$
$$z = z_{\bigcirc} \text{ on } \partial\Omega_{\bigcirc}, \tag{S47}$$
$$n^i \nabla_i z = \psi_{\bigcirc} \text{ on } \partial\Omega_{\bigcirc}. \tag{S48}$$
$$n^i \nabla_i z = \psi_{\square} \text{ on } \partial\Omega_{\square}, \tag{S49}$$

where, along the lines of Case 1a, Eqs. (S46) to (S49) fix the manifold height and slope at both the circle and square boundary.

Proceeding along the lines of Case 1a, the BVP is given by Eqs. (S42) to (S44), with Dirichlet BCs given by Eqs. (S46) and (S47), and a penalty term

$$G_\omega \equiv \frac{\alpha}{l} \left[ \langle (n^i \omega_i - \psi_{\bigcirc}) n_j \nu_\omega{}^j \rangle_{\partial\Omega_{\bigcirc}} + \langle (n^i \omega_i - \psi_{\square}) n_j \nu_\omega{}^j \rangle_{\partial\Omega_{\square}} \right], \tag{S50}$$

which enforces Eqs. (S48) and (S49).

This VP is solved in the `steady_state_no_flow` module as `variational_problem_bc_square_a`, see Fig. 2.

2. **Fixed-slope boundary conditions.**

Here, the profile of $\mathscr{M}$ is fixed at the outer boundary only, where we fix also its derivative along $n$, cf. Fig. 1. At the inner boundary, both components of the manifold gradient are fixed.

For the sake of conciseness, we discuss the VP for the rectangle-with-circle geometry of Case 3 in Section S1.8 only. We consider the BCs

Eq. (S46),

$$\nabla_i z = \phi_i \text{ on } \partial\Omega_{\bigcirc}, \tag{S51}$$
$$n^i \nabla_i z = \psi \text{ on } \partial\Omega_{\square}. \tag{S52}$$

The BVP is given by Eqs. (S42) to (S44), where we enforce Eqs. (S46) and (S51) as Dirichlet BCs and Eq. (S52) with a penalty term

$$G_\omega = \frac{\alpha}{l} \langle (n^i \omega_i - \psi) n_j \nu_\omega{}^j \rangle_{\partial\Omega_{\square}}. \tag{S53}$$

This VP is solved in the `steady_state_no_flow` module as `variational_problem_bc_square_b`, see Fig. 3.

### S3.1.2 Steady state with flows

In this Section, we will derive the variational formulation for Eqs. (9) to (12), proceeding along the same lines as Section S3.1.1.

We multiply Eqs. (18) to (21) by $\sqrt{|g|}$ and by the test functions $\nu_\sigma$, $\nu_{v\,i}$, $\nu_w$, $\nu_z$, $\nu_\omega{}^i$ and $\nu_\mu$ for the fields, $\sigma$, $v$, $w$, $z$, $\omega$ and $\mu$, respectively, take the average (S16) of both sides of each equation, and obtain

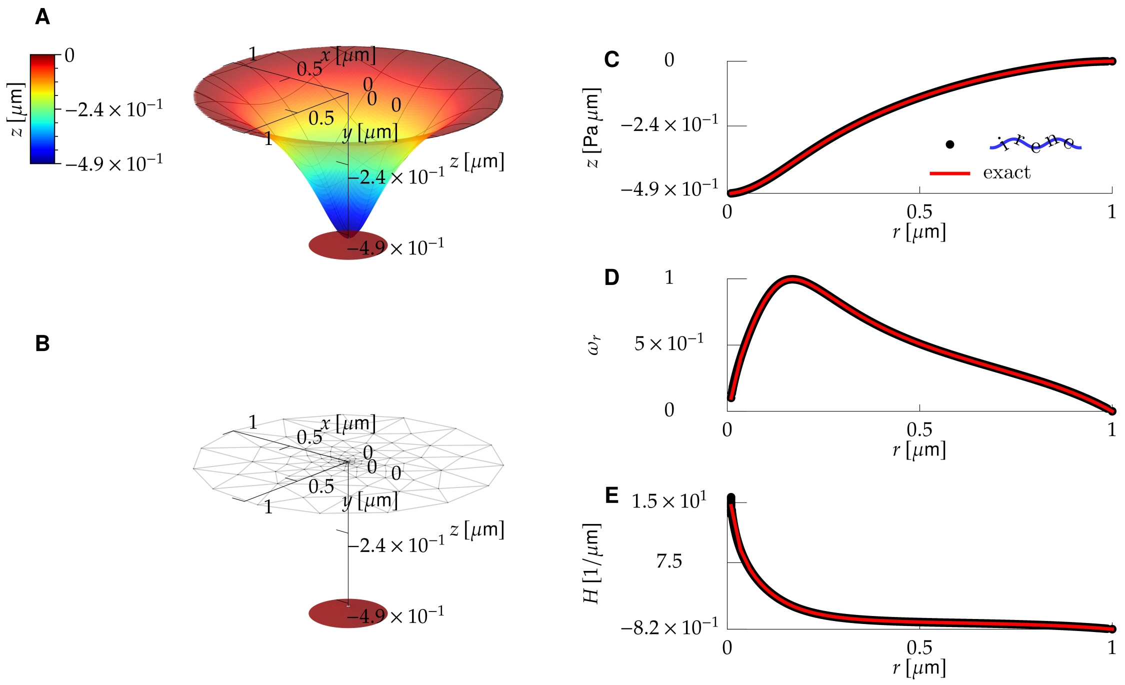


**Figure S1:** Steady state in the absence of flows for a lipidic membrane with a trans-membrane protein inclusion on a ring geometry, with fixed-height boundary conditions, Eqs. (S38) to (S41). The solution has been obtained with parameters (17) and $z_{\odot} = -0.5\,\mu\text{m}$, $z_{\bigcirc} = 0\,\mu\text{m}$, $\psi_{\odot} = -0.1$, $\psi_{\bigcirc} = 0$, $\sigma = 1\,\text{Pa}\,\mu\text{m}$, and outer-circle radius $R = 1\,\mu\text{m}$, where both circles are centered at the origin. **A**) Membrane profile $z$ (surface) and trans-membrane protein (red cone), where the color code represents the membrane height. The black curves along the surface serve as guides for the eye. **B**) Mesh and protein. For the sake of clarity, the shown mesh is coarser than the one used to produce the solution. **C**) Membrane height $z$ as a function of the radial coordinate $r$, from (black) and the numerically exact solution (red). **D**) Same as **C**, for the membrane-profile derivative $\omega_r$. **E**) Same as **C**, for the mean curvature $H$.

$$\left\langle (\nabla_i v^i - 2\mu w)\nu_\sigma \right\rangle_\Omega = 0, \tag{S54}$$

$$\left\langle \left\{ \rho \left( v^j \nabla_j v^i - 2 v^j w b^i_j - w \nabla^i w \right) - \nabla^i \sigma - \right.\right.$$
$$\left.\left. -\eta \left[ -\nabla_{\mathrm{LB}} v^i - 2 \left( b^{ij} - 2\,\mu\, g^{ij} \nabla_j w \right) + 2K v^i \right] \right\} \nu_{v\,i} \right\rangle_\Omega = 0 \tag{S55}$$

$$\left\langle \left\{ \rho v^i \left( v^j b_{ji} + \nabla_i w \right) - 2\kappa \left[ \nabla_{\mathrm{LB}} \mu - 2\mu(\mu^2 - K) \right] - 2\sigma\mu - \right.\right.$$
$$\left.\left. -2\eta \left[ (\nabla^i v^j) b_{ij} - 2w(2\mu^2 - K) \right] \right\} \nu_w \right\rangle_\Omega = 0, \tag{S56}$$

$$\left\langle \left[ w \left( \hat{N}^3 - \hat{N}^i \omega_i \right) \right] \nu_z \right\rangle_\Omega = 0, \tag{S57}$$

Eqs. (S30) and (S31),

We now integrate by parts some terms in Eqs. (S30), (S31) and (S54) to (S57). The convective and surface-tension term in the left-hand side (LHS) of Eq. (S55), and the convective and curvature term in the LHS of Eq. (S56), can be rewritten by using Eqs. (S12) and (S18) as

$$\left\langle w (\nabla^i w) \nu_{v\,i} \right\rangle_\Omega = \frac{1}{2} \left\langle [\nabla^i (w^2)] \nu_{v\,i} \right\rangle_\Omega$$
$$= \frac{1}{2} \left[ - \left\langle w^2 \nabla^i \nu_{v\,i} \right\rangle_\Omega + \left\langle n^i w^2 \nu_{v\,i} \right\rangle_{\partial\Omega} \right], \tag{S58}$$

$$\left\langle (\nabla^i \sigma) \nu_{v\,i} \right\rangle_\Omega = - \left\langle \sigma \nabla^i \nu_{v\,i} \right\rangle_\Omega + \left\langle n^i \sigma \nu_{v\,i} \right\rangle_{\partial\Omega}, \tag{S59}$$

$$\left\langle v^i (\nabla_i w) \nu_w \right\rangle_\Omega = - \left\langle w [\nabla_i (v^i \nu_w)] \right\rangle_\Omega + \left\langle n_i v^i w \nu_w \right\rangle_{\partial\Omega}, \tag{S60}$$

$$\left\langle (\nabla^i \nabla_i \mu) \nu_w \right\rangle_\Omega = - \left\langle (\nabla_i \mu) \nabla^i \nu_w \right\rangle_\Omega + \left\langle n^i (\nabla_i \mu) \nu_w \right\rangle_{\partial\Omega}, \tag{S61}$$

respectively. The viscous term in Eq. (S55) can be rewritten as

$$\left\langle \left\{ \eta \left[ -\nabla_{\mathrm{LB}} v^i - 2 \left( b^{ij} - 2\,\mu\, g^{ij} \nabla_j w \right) + 2K v^i \right] \right\} \nu_{v\,i} \right\rangle_\Omega =$$
$$2\eta \left\langle (\nabla_j d^{ij}) \nu_{v\,i} \right\rangle_\Omega = \tag{S62}$$
$$2\eta \left( - \left\langle d^{ij} \nabla_j \nu_{v\,i} \right\rangle_\Omega + \left\langle n_j d^{ij} \nu_{v\,i} \right\rangle_{\partial\Omega} \right) \tag{S63}$$

where in the first line we used Eqs. (15), (S24) and (S25), and the second line we used Eq. (S19). Combining Eqs. (S43), (S44), (S54) to (S58), (S62) and (S63), we define the variational functionals

$$F_\sigma \equiv \left\langle (\nabla_i v^i - 2\mu w) \nu_\sigma \right\rangle_\Omega, \tag{S64}$$

$$F_v \equiv \left\langle \rho \left( v^j \nabla_j v^i - 2 v^j w b^i_j \right) \nu_{v\,i} + 2\eta\, d^{ij} \nabla_j \nu_{v\,i} + \left( \frac{\rho}{2} w^2 + \sigma \right) \nabla^i \nu_{v\,i} \right\rangle_\Omega -$$
$$- \left\langle n_j \left[ g^{ij} \left( \frac{\rho}{2} w^2 + \sigma \right) + 2\eta\, d^{ij} \right] \nu_{v\,i} \right\rangle_{\partial\Omega} \tag{S65}$$

$$F_w \equiv \left\langle \left\{ \rho\, v^i v^j b_{ji} + 4\kappa\, \mu(\mu^2 - K) - 2\sigma\mu - \right.\right.$$
$$\left.\left. -2\eta \left[ (\nabla^i v^j) b_{ij} - 2w(2\mu^2 - K) \right] \right\} \nu_w - 2\kappa (\nabla^i \mu) \nabla_i \nu_w - \rho\, w \nabla_i \left( v^i \nu_w \right) \right\rangle_\Omega +$$
$$+ \left\langle \rho\, n_i v^i w \nu_w + 2\kappa n_i (\nabla^i \mu) \nu_w \right\rangle_{\partial\Omega}, \tag{S66}$$

$$F_z \equiv \left\langle \left[ w \left( \hat{N}^3 - \hat{N}^i \omega_i \right) \right] \nu_z \right\rangle_\Omega, \tag{S67}$$

where in Eq. (S65) we substituted Eqs. (S58), (S59), (S62) and (S63), and in Eq. (S66) we used Eqs. (S60) and (S61).

We will consider the following geometries and BCs:

1. **Fixed-height BCs.**

   Here, the manifold height on the whole boundary is fixed, together with its derivative along the normal $n$ at the boundary, cf. Case 1 in Section S3.1.1.

(a) **Ring geometry.**

For the geometry of Case 1 in Section S1.8, we consider the BCs

$$
\begin{aligned}
v^i &= v^i_{\odot} \text{ on } \partial\Omega_{\odot}, && \text{(S68)}\\
n^i v_i &= \chi_{\bigcirc} \text{ on } \partial\Omega_{\bigcirc}, && \text{(S69)}\\
w &= 0 \text{ on } \partial\Omega, && \text{(S70)}\\
\sigma &= \sigma_{\bigcirc} \text{ on } \partial\Omega_{\bigcirc}, && \text{(S71)}\\
z &= z_{\odot} \text{ on } \partial\Omega_{\odot}, && \text{(S72)}\\
z &= z_{\bigcirc} \text{ on } \partial\Omega_{\bigcirc}, && \text{(S73)}\\
n^i \nabla_i z &= \psi_{\odot} \text{ on } \partial\Omega_{\odot} && \text{(S74)}\\
n^i \nabla_i z &= \psi_{\bigcirc} \text{ on } \partial\Omega_{\bigcirc} && \text{(S75)}
\end{aligned}
$$

From the physical standpoint, Equations (S68) to (S71) fix the boundary values of the velocity and surface tension, while Eqs. (S72) to (S75) are fixed-height BCs, cf. Eqs. (S46) to (S49).
The resulting VP is given by

$$
\begin{aligned}
F_\sigma &= 0, && \text{(S76)}\\
F_v &= 0, && \text{(S77)}\\
F_w &= 0, && \text{(S78)}\\
F_z &= 0, && \text{(S79)}\\
&\text{Eqs. (S43) and (S44)}, && \text{(S80)}
\end{aligned}
$$

In Eqs. (S43), (S44) and (S76) to (S79), we impose Eqs. (S68) and (S70) to (S73) as Dirichlet BCs. The BCs (S69), (S74) and (S75) are enforced with the penalty method by adding, respectively, the functionals

$$
\begin{aligned}
G_v &\equiv \frac{\alpha}{l} \langle (n^i v_i - \chi_{\bigcirc}) n_j \nu_v{}^j \rangle_{\partial\Omega_{\bigcirc}}, && \text{(S81)}\\
G_\omega &\equiv \frac{\alpha}{l} \left[ \langle (n^i \omega_i - \psi_{\odot}) n_j \nu_\omega{}^j \rangle_{\partial\Omega_{\odot}} + \langle (n^i \omega_i - \psi_{\bigcirc}) n_j \nu_\omega{}^j \rangle_{\partial\Omega_{\bigcirc}} \right], && \text{(S82)}
\end{aligned}
$$

in which we used the definition (14).

This VP is solved in the `steady_state_flow` module as `variational_problem_bc_ring_1`, see Fig. S2

(b) **Square geometry.**

For the geometry of Case 3 in Section S1.8, we consider the BCs

$$
\begin{aligned}
v^1 &= v_{\sqsubset} \text{ on } \partial\Omega_{\sqsubset}, && \text{(S83)}\\
v^2 &= 0 \text{ on } \partial\Omega_{\sqsubset}, && \text{(S84)}\\
n^i v_i &= 0 \text{ on } \partial\Omega_{\bigcirc} \cup \partial\Omega_{\boxminus} && \text{(S85)}\\
n_i \Pi^{i1} &= 0 \text{ on } \partial\Omega_{\sqsupset}, && \text{(S86)}\\
w &= 0 \text{ on } \partial\Omega, && \text{(S87)}\\
\sigma &= \sigma_{\sqsupset} \text{ on } \partial\Omega_{\sqsupset}, && \text{(S88)}\\
z &= 0 \text{ on } \partial\Omega, && \text{(S89)}\\
n^i \nabla_i z &= \psi_{\blacksquare} \text{ on } \partial\Omega_{\blacksquare} && \text{(S90)}\\
n^i \nabla_i z &= \psi_{\bigcirc} \text{ on } \partial\Omega_{\bigcirc} && \text{(S91)}
\end{aligned}
$$

From the physical standpoint, Equations (S83) to (S85), (S87) and (S88) fix the boundary values of the velocity and surface tension, while Eq. (S86) enforces zero traction along the $x$ axis at outflow, $\partial\Omega_{\square_\mathrm{r}}$ [10]. Finally, Eqs. (S89) to (S91) impose fixed height, cf. Eqs. (S38) to (S41).
First, Eq. (S86) is imposed as a natural BC: By using Eqs. (S23) and (S88) we obtain

$$n_i d^{i1} = 0 \text{ on } \partial\Omega_{\square_\mathrm{r}}, \tag{S92}$$

and by substituting Eq. (S92) into the boundary term of Eq. (S65), we obtain [15, 14]

$$\begin{aligned}\left\langle \rho \left( v^j \nabla_j v^i - 2 v^j w b^i_j \right) \nu_{v\,i} + 2\eta\, d^{ij} \nabla_j \nu_{v\,i} + \left( \frac{\rho}{2} w^2 + \sigma \right) \nabla^i \nu_{v\,i} \right\rangle_\Omega - \\ - \left\langle \left( \frac{\rho}{2} w^2 + \sigma \right) n^i \nu_{v\,i} \right\rangle_{\partial\Omega} - \\ - \langle 2\eta\, n_j d^{ij} \nu_{v\,i} \rangle_{\partial\Omega_{\square_\mathrm{l}} \cup \partial\Omega_{\square_\mathrm{tb}} \cup \partial\Omega_{\bigcirc}} - \\ - \langle 2\eta\, n_j d^{i2} \nu_{v\,i} \rangle_{\partial\Omega_{\square_\mathrm{r}}} = 0.\end{aligned} \tag{S93}$$

The variational problem is thus given by Eqs. (S43), (S44), (S76), (S78), (S79) and (S93).
In such variational equations, Eqs. (S83), (S84) and (S87) to (S89) are imposed as Dirichlet BCs, while Eqs. (S85), (S90) and (S91) are enforced with the penalty method, by adding to the VP the functionals

$$G_v \equiv \frac{\alpha}{l} \langle n^i v_i n_j \nu_v{}^j \rangle_{\partial\Omega_{\bigcirc} \cup \partial\Omega_{\square_\mathrm{tb}}}, \tag{S94}$$

$$G_\omega \equiv \frac{\alpha}{l} \left[ \langle (n^i \omega_i - \psi_{\square}) n_j \nu_\omega{}^j \rangle_{\partial\Omega_{\square}} + \langle (n^i \omega_i - \psi_{\bigcirc}) n_j \nu_\omega{}^j \rangle_{\partial\Omega_{\bigcirc}} \right], \tag{S95}$$

in which we used Eq. (14).
This VP is solved in the `steady_state_flow` module as `variational_problem_bc_square_a`, see Fig. S4.

2. **Fixed-slope BCs.**

   (a) **Ring geometry.**
   For the geometry of Case 1 in Section S1.8, we consider the BCs

Eqs. (S68), (S69) and (S73),

$$w = 0 \text{ on } \partial\Omega_{\bigcirc}, \tag{S96}$$

$$\sigma = \sigma_{\bigcirc} \text{ on } \partial\Omega_{\bigcirc}, \tag{S97}$$

$$\nabla_i z = \psi_{i\,\odot} \text{ on } \partial\Omega_{\odot}, \tag{S98}$$

$$\nabla_i z = \psi_{i\,\bigcirc} \text{ on } \partial\Omega_{\bigcirc}, \tag{S99}$$

where Eqs. (S73), (S98) and (S99) impose fixed slope, cf. Eqs. (S46), (S51) and (S52).
The resulting BVP is given by Eqs. (S42) to (S44) and (S76) to (S79), where Eqs. (S68), (S73), (S96) and (S97) are imposed as Dirichlet BCs, and Eqs. (S69), (S98) and (S99) are enforced by adding the penalty terms in Eqs. (S81) and (S82), in which we used Eq. (14).
This VP is solved in the `steady_state_flow` module as `variational_problem_bc_ring_2`, see Fig. S3.

   (b) **Square geometry.**
   For the geometry of Case 3 in Section S1.8, we consider the BCs

Eqs. (S83), (S84), (S86) and (S88)

$$v^i = 0 \text{ on } \partial\Omega_{\bigcirc}, \tag{S100}$$
$$n^i v_i = 0 \text{ on } \partial\Omega_{\square}, \tag{S101}$$
$$w = 0 \text{ on } \partial\Omega_{\square}, \tag{S102}$$
$$z = 0 \text{ on } \partial\Omega_{\square}, \tag{S103}$$
$$\nabla_i z = \phi_i \text{ on } \partial\Omega_{\bigcirc}, \tag{S104}$$
$$n^i \nabla_i z = \psi \text{ on } \partial\Omega_{\square}. \tag{S105}$$

Proceeding along the lines of Case 1b, Eq. (S86) is enforced as a natural BC, and we obtain Eq. (S93). As a result, the VP is given by Eqs. (S43), (S44), (S76), (S78), (S79) and (S93).

In this VP, Eqs. (S83), (S84), (S88), (S100) and (S102) to (S104) are imposed as Dirichlet BCs, Eq. (S86) as a natural BC, and Eqs. (S101) and (S105) by adding the penalty terms

$$G_v \equiv \frac{\alpha}{l} \langle n^i v_i n_j \nu_v{}^j \rangle_{\partial\Omega_{\square}}, \tag{S106}$$
$$G_\omega \equiv \frac{\alpha}{l} \langle (n^i \omega_i - \psi) n_j \nu_\omega{}^j \rangle_{\partial\Omega_{\square}}, \tag{S107}$$

where we substituted Eq. (14).

This VP is solved in the `steady_state_flow` module as `variational_problem_bc_square_b`, see Fig. 4.

## S3.2 Dynamics

### S3.2.1 Fixed manifold

In this Section, we will discuss the solution of Eqs. (23) and (24) for two geometries and BCs:

1. **Rectangular geometry.**

   For the geometry of Case 2 in Section S1.8, we consider, at any time $t$, the BCs

$$v^i = v^i_{\square} \text{ on } \partial\Omega_{\square}, \tag{S108}$$
$$v^i = 0 \text{ on } \partial\Omega_{\square}, \tag{S109}$$
$$n_j \Pi^{ji} = 0 \text{ on } \partial\Omega_{\square}, \tag{S110}$$
$$\sigma = 0 \text{ on } \partial\Omega_{\square}, \tag{S111}$$

   where Eq. (S110) enforces zero traction [10].

   The BCs relative to the time variable are

$$v^i(\boldsymbol{x}, t=0) = v^i_0(\boldsymbol{x}), \tag{S112}$$
$$\sigma(\boldsymbol{x}, t=0) = \sigma_0(\boldsymbol{x}), \tag{S113}$$

   which are intended to hold for all $\boldsymbol{x} \in \Omega$.

   In what follows, we discretize time by setting

$$t^n \equiv n\,\Delta t, \tag{S114}$$

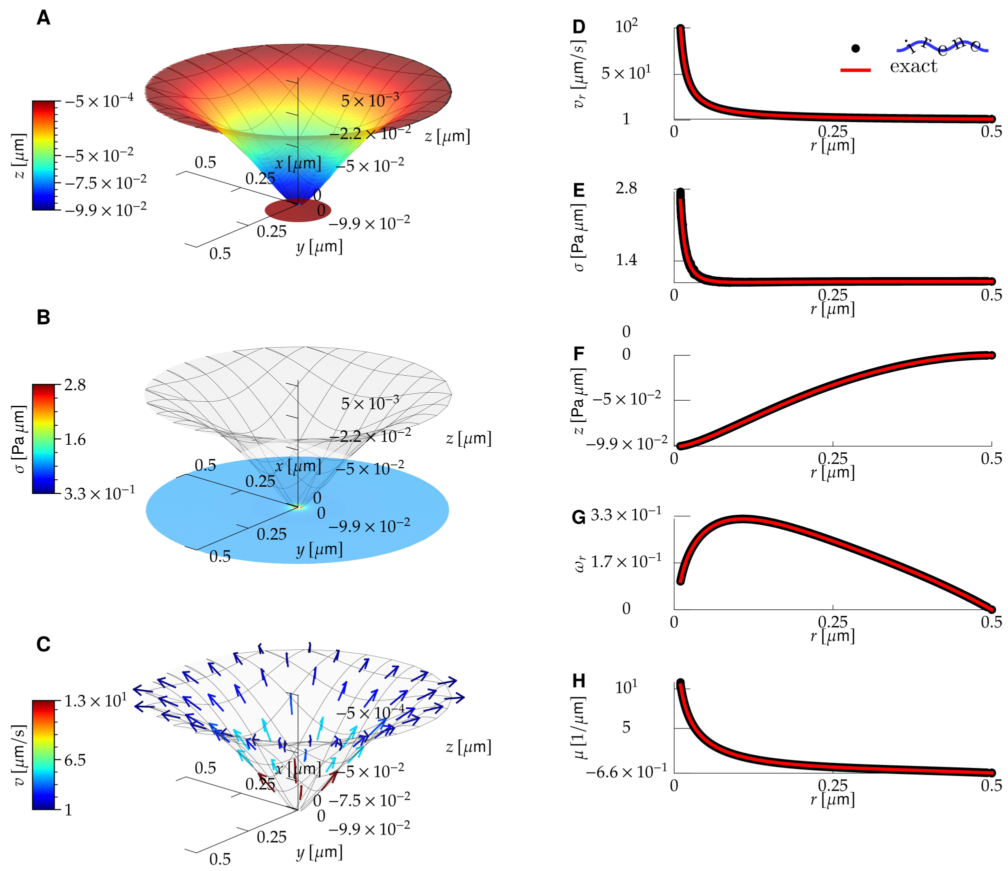


**Figure S2:** Steady state in the presence of flows for a lipidic membrane on a circular geometry with a with a trans-membrane protein inclusion, which acts as a source of membrane flow. Here we impose fixed-height boundary conditions, Eqs. (S38) to (S41). The solution is obtained with parameters (17), $v^i_{\odot} = 10^2\, \hat{x}^i\ \mu\text{m}/s$, $\chi_{\bigcirc} = 2\,\mu\text{m}/s$, $\sigma_{\bigcirc} = 1\,\text{Pa}\,\mu\text{m}$, $z_{\odot} = -0.1\,\mu\text{m}$, $z_{\bigcirc} = 0$, $\psi_{\odot} = -0.1$, $\psi_{\bigcirc} = 0$, and outer ring radius $R = 0.5\,\mu\text{m}$, where both circles are centered at the origin. **A**) Membrane profile $z$. **B**) Surface tension $\sigma$. **C**) Tangential velocity $v$, displayed on top of the surface of **A**. The direction of the velocity field is represented by the arrows, and the modulus by the arrow color. In **D-H**, we show the solution for $v$, $\sigma$, $z$, $\omega_r$ and $\mu$ from and from the numerically exact solution.

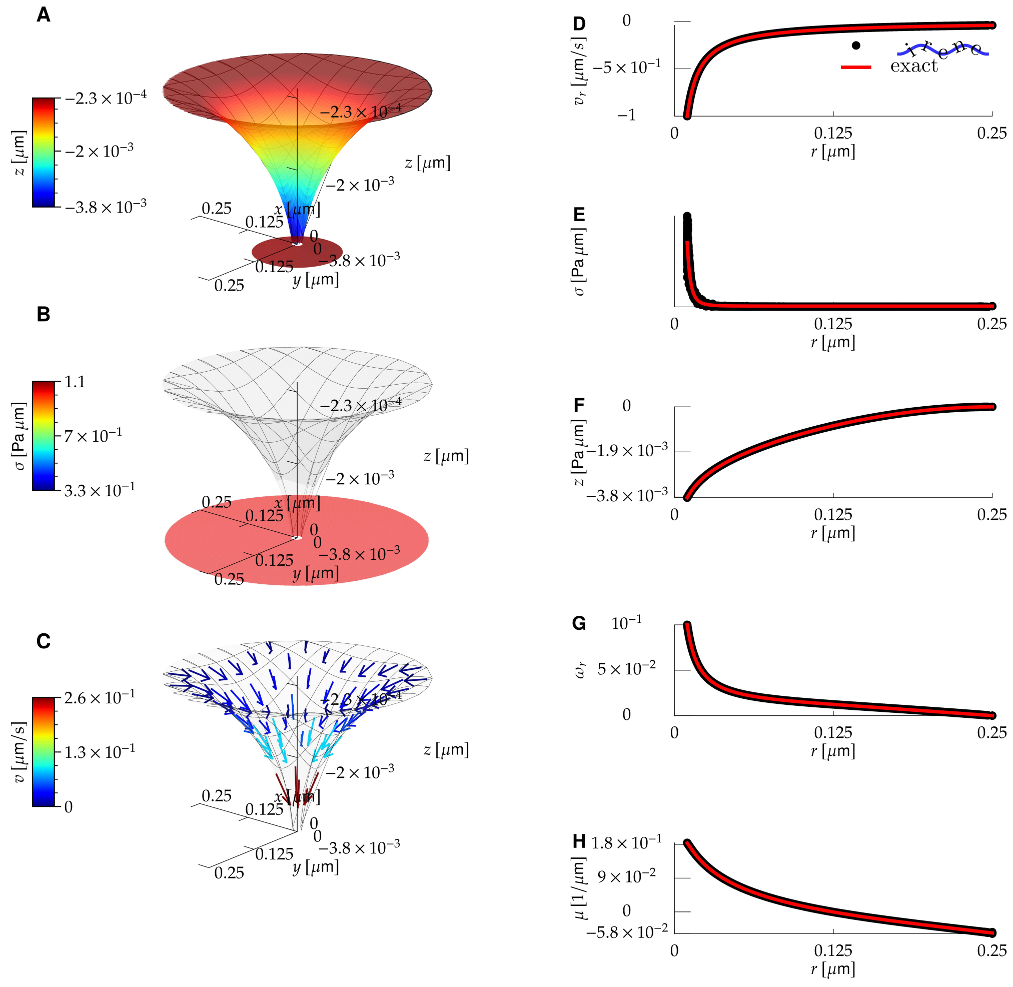


**Figure S3:** Steady state in the presence of flows for a lipidic membrane on a ring geometry, with a transmembrane protein inclusion, which acts as a sink of membrane flows. Here, we impose fixed-slope boundary conditions (S68), (S69), (S73) and (S96) to (S99). The solution is obtained with parameters (17), $v^i_{\odot} = -\hat{x}^i\ \mu\text{m}/s$, $v^i_{\bigcirc} = -4.02\,\hat{x}^i \times 10^{-2}\ \mu\text{m}/s$, $\sigma_{\bigcirc} = 1\,\text{Pa}\,\mu\text{m}$, $z_{\bigcirc} = 0$, $\psi_{i\,\odot} = 0.1\,\hat{x}^i$, $\psi_{i\,\bigcirc} = 0$. Ring geometry is the same as in Fig. S1, with $R = 0.25\,\mu\text{m}$. Panels follow the same notation as Fig. S2.

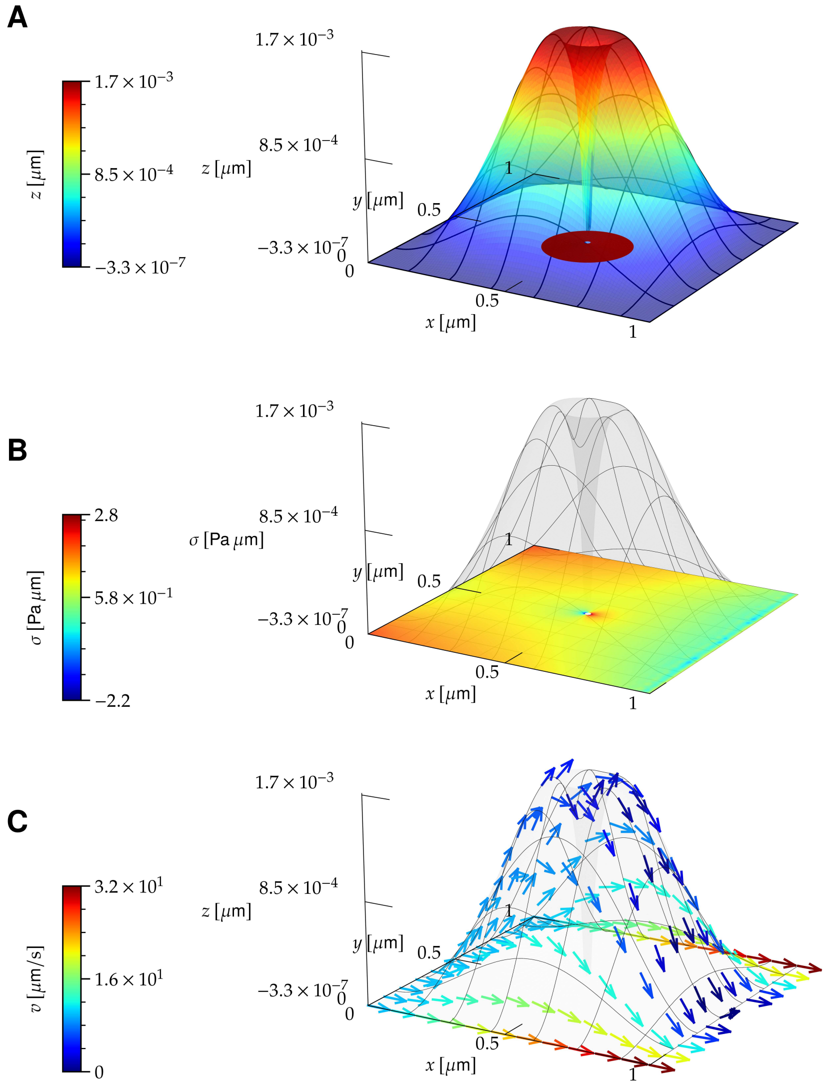


**Figure S4:** Steady state in the presence of flows for a lipidic membrane with a trans-membrane protein on a square geometry, with fixed-height boundary conditions, Eqs. (S83) to (S91). The solution has been obtained with parameters (17), $v_{\square} = 10\,\mu\mathrm{m}/s$, $\sigma_{\square} = 1\mathrm{Pa}\,\mu\mathrm{m}$, $\psi_{\square} = 0$, $\psi_{\bigcirc} = -0.1$, rectangle and obstacle geometry is the same as in Fig. 2. Panels follow the same notation as Fig. S2.

where $n = 0, 1, \cdots$, and set

$$
\begin{aligned}
\sigma^n \equiv & \sigma(t^n), \\
\sigma^{n-1/2} \equiv & \sigma\left(\frac{t^n + t^{n-1}}{2}\right), \\
\sigma^{n-3/2} \equiv & \sigma\left(\frac{t^{n-1} + t^{n-2}}{2}\right),
\end{aligned}
\tag{S115}
$$

and similarly for other quantities.

We will now rewrite the BVP in discrete form, yielding a set of equations exact to $O(\Delta t)$.

The discrete form of Eqs. (23) and (24) is

$$\nabla_i v^{n,i} = 0, \tag{S116}$$

$$
\begin{aligned}
\rho\left(\frac{v^{n,i} - v^{n-1,i}}{\Delta t} + \frac{3}{2} v^{n-1,j} \nabla_j v^{n-1,i} - \frac{1}{2} v^{n-2,j} \nabla_j v^{n-2,i}\right) = \\
= \nabla^i \sigma^{n-1/2} + {f_\eta}^i\left(\frac{v^n + v^{n-1}}{2}\right),
\end{aligned}
\tag{S117}
$$

where in Eq. (S117) we discretized the nonlinear Navier-Stokes (NS) term with the Crank Nicolson (CN) method [17], which improves the stability of the solution scheme [14]. Also, we wrote explicitly the dependence of the viscous force in Eqs. (S24) and (S25) on the velocity field.

The discrete version of the BCs (S108) to (S113), is

$$v^{n,i} = {v_{\sqsubset}}^{n,i} \text{ on } \partial\Omega_{\sqsubset}, \tag{S118}$$

$$v^{n,i} = 0 \text{ on } \partial\Omega_{\sqcup}, \tag{S119}$$

$$n_j \Pi^{ji}\left(\frac{v^n + v^{n-1}}{2}, \sigma^{n-1/2}\right) = 0 \text{ on } \partial\Omega_{\sqsupset}, \tag{S120}$$

$$\sigma^{n-1/2} = 0 \text{ on } \partial\Omega_{\sqsupset}, \tag{S121}$$

$$v^{0,i} = v_0^i(\boldsymbol{x}), \tag{S122}$$

$$\sigma^{-1/2} = \sigma_0(\boldsymbol{x}). \tag{S123}$$

It is important to point out that in Eqs. (S116) to (S123), we solve for the velocity at integer time steps $n = 0, 1, \cdots$, and for the surface tension at semi-integer steps $n = 1/2, 3/2, \cdots$ [14].

In order to solve Eqs. (S116) and (S117) in a stable and efficient way, we will use a splitting scheme [14], in which Eq. (S117) and Eq. (S116) are solved separately. Among the proposed splitting schemes [18, 19], we will employ the incremental pressure correction scheme (IPCS) [20], which we will detail in the following—see [14, 20] for details. We observe that IPCS has been developed for the NS equations, which involve the pressure field, whose analog in our analysis is the surface-tension field; in what follow we will thus use the terms 'pressure' to denote the surface tension, in order to stick with the original terminology.

For any given $n$, we set

$$\sigma^* \equiv \sigma^{n-3/2}, \tag{S124}$$

and introduce the auxiliary velocity $\overline{v}$, which represents an approximation of the solution $v^n$. We will then split the BVPs of Eqs. (S116) to (S121) into the following steps:

(a) **Approximated velocity.**
We consider the following BVP for $\overline{v}$:

$$\rho\left[\frac{\overline{v}^i - v^{n-1,i}}{\Delta t} + \left(\frac{3}{2}v^{n-1,j} - \frac{1}{2}v^{n-2,j}\right)\nabla_j V^i\right] = \nabla^i\sigma^* + {f_\eta}^i(V), \tag{S125}$$

$$\overline{v}^i = {v_{\text{◧}}}^{n,i} \text{ on } \partial\Omega_{\text{◧}}, \tag{S126}$$

$$\overline{v}^i = 0 \text{ on } \partial\Omega_{\text{⬓}}, \tag{S127}$$

$$n_j \Pi^{ji}(V, \sigma^*) = 0 \text{ on } \partial\Omega_{\text{◨}}, \tag{S128}$$

where

$$V^i \equiv \frac{\overline{v}^i + v^{n-1,i}}{2}. \tag{S129}$$

Equation (S125) is obtained from the original BVP of Eqs. (S117) to (S120) by replacing the surface tension with the known field $\sigma^*$, and the velocity field $v$ with either $\overline{v}$ or $V$. The resulting solution $\overline{v}$ thus constitutes an approximation for the exact velocity field $v$, and the two differ by $O(\Delta t)$.

(b) **Pressure correction.**
Subtracting Eqs. (S117) and (S125), we obtain

$$\frac{\rho}{\Delta t}(v^{n,i} - \overline{v}^i) = -\nabla^i\phi + O(\Delta t), \tag{S130}$$

where the surface-tension increment is defined as

$$\phi \equiv \sigma^* - \sigma^{n-1/2}. \tag{S131}$$

By taking the covariant derivative of Eq. (S130) and neglecting $O(\Delta t)$, we obtain

$$\nabla_i\nabla^i\phi = \frac{\rho}{\Delta t}\nabla_i\overline{v}^i \tag{S132}$$

where, unlike $v^n$, the covariant divergence of $\overline{v}$ is not equal to zero. Equation (S132) is a Poisson-like equation [16] for $\phi$, for which we will now work out the BCs.
First, by multiplying Eq. (S130) by $n_i$, using Eqs. (S118), (S119), (S126) and (S127), and neglecting $O(\Delta t)$, we obtain the Neumann BCs

$$n^i\nabla_i\phi = 0 \text{ on } \partial\Omega_{\text{⊏}}. \tag{S133}$$

Second, Eqs. (S121), (S124) and (S131) imply

$$\phi = 0 \text{ on } \partial\Omega_{\text{◨}}. \tag{S134}$$

Equations (S132) to (S134) constitute a Poisson-like BVP which determines the pressure difference $\phi$. Once $\phi$ is known, the surface tension $\sigma^{n-1/2}$ is obtained by means of Eq. (S131).

(c) **Velocity.** Given that $\overline{v}$ and $\phi$ are known from Cases 1a and 1b, the velocity field is obtained, neglecting $O(\Delta t)$ terms, from Eq. (S130).

We will now discuss the variational formulation of the BVPs in Cases 1a to 1c [14].

(a) **Approximated velocity.**
We multiply Eq. (S125) by $\sqrt{|g|}\,\nu_{\overline{v}i}$, integrate, and obtain

$$\begin{aligned}\left\langle \rho\left[\frac{\overline{v}^i - v^{n-1,i}}{\Delta t} + \left(\frac{3}{2}v^{n-1,j} - \frac{1}{2}v^{n-2,j}\right)\nabla_j V^i\right]\nu_{\overline{v}i}\right\rangle_\Omega &+ \\ + \left\langle \sigma^*\nabla^i\nu_{\overline{v}i}\right\rangle_\Omega - \left\langle n^i\sigma^*\nu_{\overline{v}i}\right\rangle_{\partial\Omega} &+ \\ +2\eta\left[\left\langle d^{ij}(V)\nabla_j\nu_{\overline{v}i}\right\rangle_\Omega - \left\langle n_j d^{ij}(V)\nu_{\overline{v}i}\right\rangle_{\partial\Omega}\right] &= 0,\end{aligned} \tag{S135}$$

where we used Eqs. (S24), (S59) and (S63), and we wrote explicitly the velocity dependence of the rate-of-deformation tensor (S22).

By using Eqs. (S23) and (S121), we enforce the BC (S128) as a natural BC in Eq. (S135), and obtain

$$\begin{aligned}\left\langle \rho \left[ \frac{\overline{v}^i - v^{n-1,i}}{\Delta t} + \left( \frac{3}{2} v^{n-1,j} - \frac{1}{2} v^{n-2,j} \right) \nabla_j V^i \right] \nu_{\overline{v}i} \right\rangle_\Omega + \\ + \left\langle \sigma^* \nabla^i \nu_{\overline{v}i} + 2\eta\, d^{ij}(V) \nabla_j \nu_{\overline{v}i} \right\rangle_\Omega - \\ - \left\langle n^i \sigma^* \nu_{\overline{v}i} \right\rangle_{\partial\Omega} - 2\eta \langle n_j d^{ij}(V) \nu_{\overline{v}i} \rangle_{\partial\Omega_{\square} \cup \partial\Omega_{\square}} = 0,\end{aligned} \tag{S136}$$

which is solved for $v$ with the Dirichlet BCs (S126) and (S127).

(b) **Pressure correction.**

Proceeding along the same lines for Eq. (S132), we obtain

$$\left\langle (\nabla^i \phi) \nabla_i \nu_\phi \right\rangle_\Omega + \frac{\rho}{\Delta t} \left\langle (\nabla_i \overline{v}^i) \nu_\phi \right\rangle_\Omega - \left\langle n^i (\nabla_i \phi) \nu_\phi \right\rangle_{\partial\Omega} = 0, \tag{S137}$$

where $\nu_\phi$ is the test function related to $\phi$, and we used Eq. (S18).

We enforce Eq. (S133) as a natural BC in Eq. (S137), and obtain the VP

$$\left\langle (\nabla^i \phi) \nabla_i \nu_\phi \right\rangle_\Omega + \frac{\rho}{\Delta t} \left\langle (\nabla_i \overline{v}^i) \nu_\phi \right\rangle_\Omega - \langle n^i (\nabla_i \phi) \nu_\phi \rangle_{\partial\Omega_{\square}} = 0, \tag{S138}$$

which we solve for $\phi$ with the Dirichlet BC (S134).

(c) **Velocity.**

Proceeding along the same lines for Eq. (S130) and neglecting $O(\Delta t)$, we obtain

$$\left\langle \left[ \frac{\rho}{\Delta t} (v^{n,i} - \overline{v}^i) + \nabla^i \phi \right] \nu_{vi} \right\rangle_\Omega = 0, \tag{S139}$$

which is solved for $v$.

We iterate in time by solving for $\overline{v}$, $\phi$ and $v^n$ with Cases 1a to 1c at each time step $t_n$, obtaining the surface tension $\sigma^{n-1/2}$ from Eq. (S131), and then setting, at the next time step, $v^n \to v^{n-1}$, $v^{n-1} \to v^{n-2}$ and $\sigma^{n-1/2} \to \sigma^{n-3/2}$.

This dynamics is solved in the `channel_with_cylinder_curved_crank_nicholson_discretization` module as `channel_with_cylinder_curved_crank_nicholson_discretization_square_no_circle`, see Fig. S5.

2. **Rectangle-with-circle geometry.**

For the geometry of Case 3 in Section S1.8, we consider, at any given $t$, the BCs

$$\begin{aligned}\text{Eqs. (S108) to (S111)}, \\ v^i = 0 \text{ on } \partial\Omega_{\circ'},\end{aligned} \tag{S140}$$

and the BCs relative to the time variable, Eqs. (S112) and (S113).

In what follows, we will sketch the result for the VPs, which can be derived along the lines of Case 1. At each time step we obtain the VPs

(a) **Approximated velocity.**

We solve

$$\left\langle \rho \left[ \frac{\overline{v}^i - v^{n-1,i}}{\Delta t} + \left( \frac{3}{2} v^{n-1,j} - \frac{1}{2} v^{n-2,j} \right) \nabla_j V^i \right] \nu_{\overline{v}i} \right\rangle_\Omega + \\ + \left\langle \sigma^* \nabla^i \nu_{\overline{v}i} + 2\eta \, d^{ij}(V) \nabla_j \nu_{\overline{v}i} \right\rangle_\Omega - \\ - \left\langle n^i \sigma^* \nu_{\overline{v}i} \right\rangle_{\partial\Omega} - 2\eta \left\langle n_j d^{ij}(V) \nu_{\overline{v}i} \right\rangle_{\partial\Omega_{\sqsubset} \cup \partial\Omega_{\circ}} = 0, \tag{S141}$$

in which we enforced Eq. (S128), which we combined with Eqs. (S23), (S121) and (S124), as a natural BC. We solve Eq. (S141) for $\overline{v}$ with Dirichlet BCs (S108), (S109), (S111) and (S140).

(b) **Pressure correction.**
We obtain the VP (S138), in which we enforced (S133) and

$$n^i \nabla_i \phi = 0 \text{ on } \partial\Omega_{\circ}. \tag{S142}$$

as natural BCs, and which we solve for $\phi$ with BC (S134).

(c) **Velocity.**
We solve the VP (S139) for $v$.

This dynamics is solved in the `channel_with_cylinder_curved_crank_nicholson_discretization` module as `channel_with_cylinder_curved_crank_nicholson_discretization_square`, see Fig. S6.

### S3.2.2 Moving manifold

In this Section we will consider the solution of Eqs. (9) to (12), combined with the definitions (14) and (15). We consider the geometry of Case 3 in Section S1.8, and, for any time $t$, the BCs

$$\text{Eqs. (S46), (S47), (S86), (S101), (S102) and (S108),}$$

$$\sigma = 0 \text{ on } \partial\Omega_{\sqsupset}, \tag{S143}$$

$$n^i v_i = 0 \text{ on } \partial\Omega_{\circ}, \tag{S144}$$

$$w = 0 \text{ on } \partial\Omega_{\circ}, \tag{S145}$$

$$n^i \nabla_i z = \psi \text{ on } \partial\Omega, \tag{S146}$$

where Eqs. (S46), (S47) and (S146) correspond to the fixed-height BCs of Case 1 in Section S3.1.1. The BCs relative to the temporal variable are, for all $\boldsymbol{x} \in \Omega$,

$$\text{Eqs. (S112) and (S113),}$$

$$w(\boldsymbol{x}, t = 0) = w_0(\boldsymbol{x}), \tag{S147}$$

$$z(\boldsymbol{x}, t = 0) = z_0(\boldsymbol{x}). \tag{S148}$$

Proceeding along the lines of Section S3.2.1, we introduce the definitions (S114), (S115), (S124)

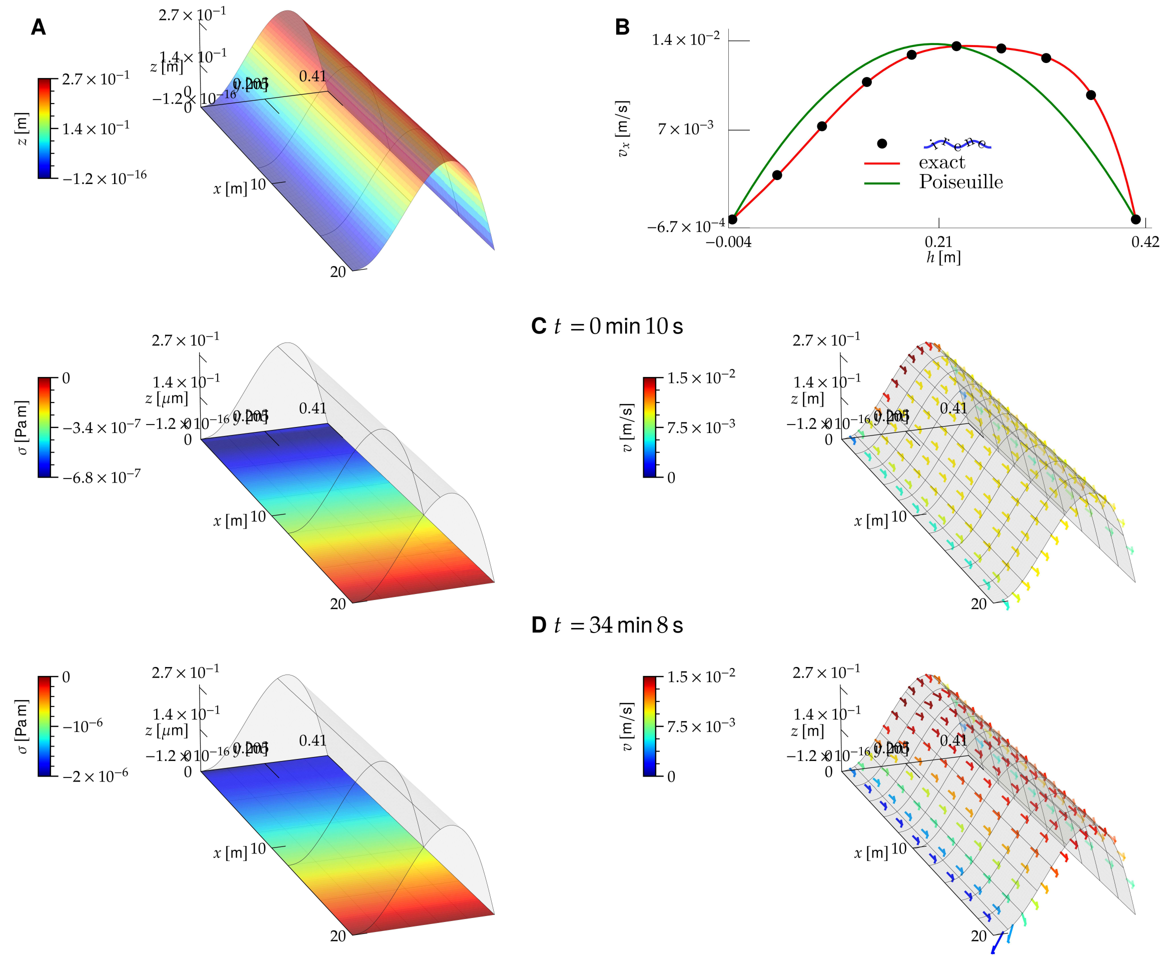


**Figure S5:** Dynamics of laminar air flow on a macroscopic, curved channel, with boundary conditions (S108) to (S111). The solution has been obtained with, $v_{\square}^{1} = 6 \times 10^{-2}\, y(y-h)/h^2$ m/s, $v_{\square}^{2} = 0$, and the dynamics has been solved for a total time $T \sim 34$ min, with $N_{\rm s} = 2048$ time steps. Dimensions of the rectangular channel are $L = 20$ m, $h = 0.41$ m [21]. Model parameters are given by (25). The inflow velocity profile $v_{\square}$ is given by the Poiseuille-flow solution on a flat manifold [10]. The rectangle height, $h$, has been taken from the FEAT2D DFG 2D-3 benchmark for a flow around a cylinder [21]. We chose the rectangle length $L$ to be large enough, in such a way that the outflow velocity profile, at $x = L$, is not affected by the inflow profile, and coincides with the free-flow profile at steady state. **A**) Manifold profile, $z$. **B**) Component along the $x$ axis of the velocity $v$ at the right boundary of the rectangular channel, $x = L$, as a function of $y$. Solution from [illegible] (black dots), exact solution (red curve) and Poiseuille-flow solution on a flat manifold (green curve). **C**) Surface tension (left) and velocity (right) profiles at an early time. The direction of the velocity field is represented by the arrows, and the modulus by the arrow color. **D**) Same as **C**, at a later time, at which the solution reached steady state.

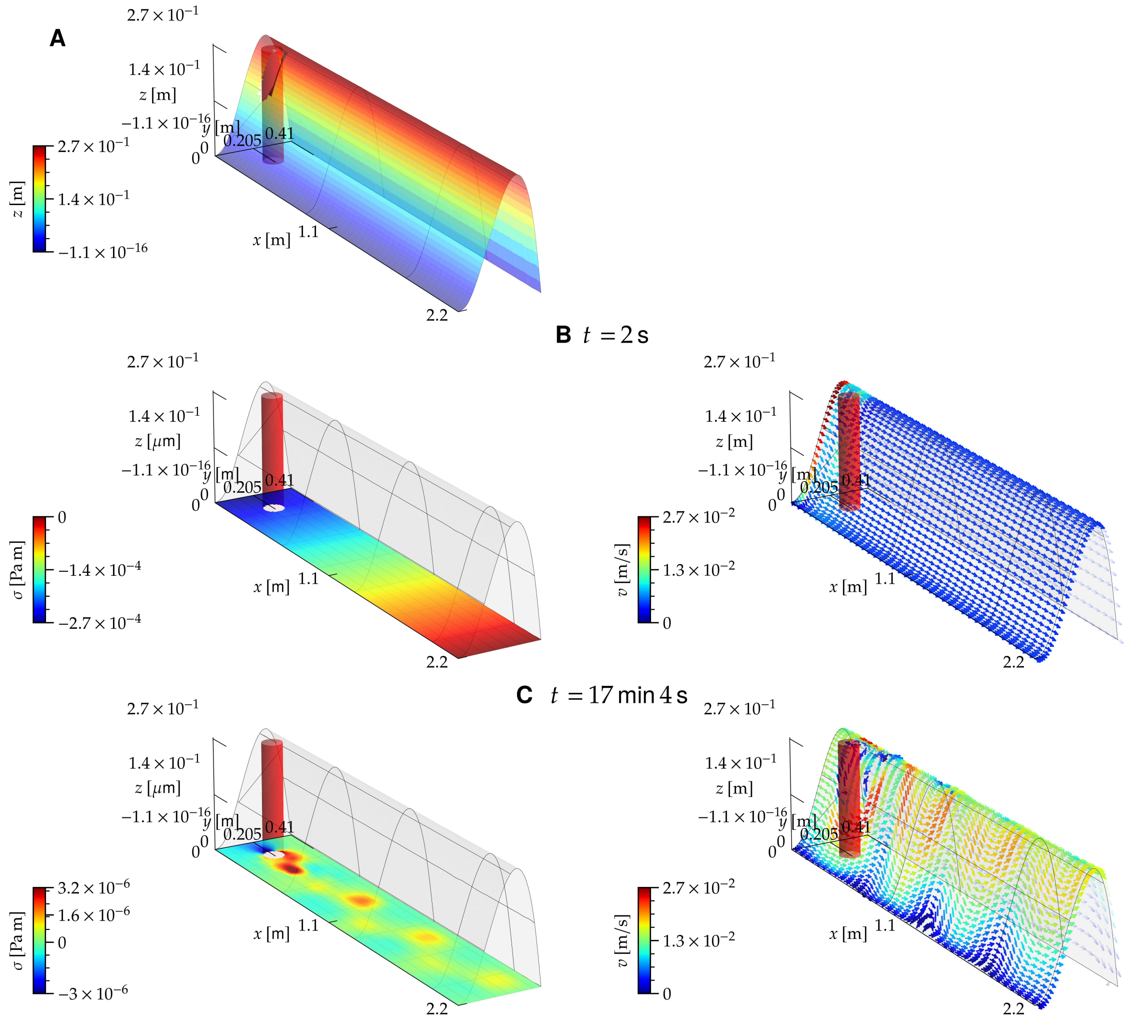


**Figure S6:** Dynamics of turbulent air flow on a macroscopic, curved channel with an obstacle (red cylinder), with boundary conditions (S108) to (S111) and (S140). The solution has been obtained with the same $v^i_{\square}$ as in Fig. S5, and the dynamics has been solved for a total time $T \sim 17\,\mathrm{min}$, with $N_\mathrm{s} = 2048$ time steps. Model parameters are given by (25), $L = 2.2\,\mathrm{m}$, $h = 0.41\,\mathrm{m}$, and the obstacle radius is $r = 0.05\,\mathrm{m}$. The dimensions of the rectangle and of the obstacle have been taken from the FEAT2D DFG 2D-3 benchmark for a flow around a cylinder [21]. Panels **A**, **B** and **C** follow the same notation, respectively, as panels **A**, **C** and **D** of Fig. S5.

and (S131), and we discretize time along the lines of Eqs. (S116) and (S117):

$$
\begin{aligned}
\nabla_i^{n-1/2} v^{n,i} - 2\mu^{n-1/2} w^n =& 0, && \text{(S149)}\\
\rho\Big(\frac{v^{n,i}-v^{n-1,i}}{\Delta t} + \frac{3}{2} v^{n-1,j}\nabla_j^{n-1/2} v^{n-1,i} - \frac{1}{2} v^{n-2,j}\nabla_j^{n-1/2} v^{n-2,i} -&\\
-2 v^{n-1,j} w^{n-1} b^{n-1/2,i}_{\phantom{n-1/2,i}j} - w^{n-1}\nabla^{n-1/2,i} w^{n-1}\Big) =&\\
= \nabla^{n-1/2,i}\sigma^{n-1/2} + f_\eta{}^i\left(\frac{v^n+v^{n-1}}{2}, \frac{w^n+w^{n-1}}{2}, \omega^{n-1/2}, \mu^{n-1/2}\right),& && \text{(S150)}\\
\rho\Big(\frac{w^n-w^{n-1}}{\Delta t} + v^{n-1,i} v^{n-1,j} b^{n-1/2}_{ji} + \frac{3}{2} v^{n-1,i}\nabla_i^{n-1/2} w^{n-1} - \frac{1}{2} v^{n-2,i}\nabla_i^{n-1/2} w^{n-2}\Big) =&\\
f_\kappa(\omega^{n-1/2}, \mu^{n-1/2}) + 2\sigma^{n-1/2}\mu^{n-1/2} + \mathfrak{f}_\eta\left(\frac{v^n+v^{n-1}}{2}, \frac{w^n+w^{n-1}}{2}, \omega^{n-1/2}, \mu^{n-1/2}\right),& && \text{(S151)}\\
\frac{z^{n-1/2}-z^{n-3/2}}{\Delta t} =&\\
= w^{n-1}\left(\hat{N}^{n-1/2,3} - \hat{N}^{n-1/2,i}\omega_i^{n-1/2}\right),& && \text{(S152)}\\
\text{Eqs. (14) and (15).}&
\end{aligned}
$$

The discrete version of the BCs (S46), (S47), (S86), (S101), (S102), (S108) and (S143) to (S146) is

$$
\begin{aligned}
v^{n,i} =& v^i_{\square} \text{ on } \partial\Omega_{\square}, && \text{(S153)}\\
n^{n-1/2,i}\Pi^{n-1/2,1}_{\phantom{n-1/2,1}i}\left(\frac{v^n+v^{n-1}}{2}, \frac{w^n+w^{n-1}}{2}, \sigma^{n-1/2}\right) =& 0 \text{ on } \partial\Omega_{\square} && \text{(S154)}\\
w^n =& 0 \text{ on } \partial\Omega, && \text{(S155)}\\
n_i^{n-1/2} v^{n,i} =& 0 \text{ on } \partial\Omega_{\square} \cup \partial\Omega_{\circ}, && \text{(S156)}\\
\sigma^{n-1/2} =& 0 \text{ on } \partial\Omega_{\square}, && \text{(S157)}\\
z^{n-1/2} =& z_{\square} \text{ on } \partial\Omega_{\square}, && \text{(S158)}\\
z^{n-1/2} =& z_{\circ} \text{ on } \partial\Omega_{\circ}, && \text{(S159)}\\
n^{n-1/2,i}\nabla_i^{n-1/2} z =& \psi \text{ on } \partial\Omega, && \text{(S160)}
\end{aligned}
$$

and the discrete version of the time BCs (S112), (S113), (S147) and (S148) is

$$
\begin{aligned}
v^{0,i} =& v_0^i(\boldsymbol{x}), && \text{(S161)}\\
w^0 =& w_0(\boldsymbol{x}), && \text{(S162)}\\
\sigma^{-1/2} =& \sigma_0(\boldsymbol{x}), && \text{(S163)}\\
z^0 =& z_0(\boldsymbol{x}). && \text{(S164)}
\end{aligned}
$$

In Eqs. (S149) to (S152), we wrote explicitly the dependence of the forces (S24), (S26) and (S27) on the velocity fields, $\omega$ and $\mu$, and we denote by

$$\nabla^{n-1/2} \tag{S165}$$

the covariant derivative obtained with $z = z^{n-1/2}$, and similarly for all other quantities, such as $b^{n-1/2}$. Importantly, in Eqs. (S149) to (S151) we chose a time discretization scheme where velocities are evaluated at integer time steps, and the surface tension and the manifold shape at semi-integer time steps [14]. This scheme proved to be stable in all the application which we considered, including those with a turbulent behavior—see for example Fig. 5.

We will now discuss the splitting scheme, proceeding along the derivation of Section S3.2.1. We introduce approximated tangential and normal velocities, $\overline{v}$ and $\overline{w}$, respectively, and set Eq. (S129) and

$$W \equiv \frac{\overline{w} + w^{n-1}}{2}. \tag{S166}$$

In what follows, we will extend the IPCS splitting scheme [20] discussed in Section S3.2.1 to solve Eqs. (S149) to (S152), by including one additional step to solve for the manifold shape:

1. **Approximated velocities.**

   Let us consider an approximated tangential and normal velocity, $\overline{v}$ and $\overline{w}$, which satisfy the following BVPs:

$$\rho\Big[\frac{\overline{v}^i - v^{n-1,i}}{\Delta t} + \Big(\frac{3}{2}v^{n-1,j} - \frac{1}{2}v^{n-2,j}\Big)\nabla_j^{n-1/2}V^i - 2V^j W b^{n-1/2,i}{}_j - W\nabla^{n-1/2,i}W\Big] = \\ = \nabla^i\sigma^{*n-1/2} + f_\eta{}^i\left(V, W, \omega^{n-1/2}, \mu^{n-1/2}\right), \tag{S167}$$

$$\rho\Big[\frac{\overline{w} - w^{n-1}}{\Delta t} + V^i V^j b_{ji}^{n-1/2} + \Big(\frac{3}{2}v^{n-1,i} - \frac{1}{2}v^{n-2,i}\Big)\nabla_i^{n-1/2}W\Big] = \\ f_\kappa(\omega^{n-1/2}, \mu^{n-1/2}) + 2\sigma^*\mu^{n-1/2} + \mathfrak{f}_\eta\left(V, W, \omega^{n-1/2}, \mu^{n-1/2}\right) \tag{S168}$$

   with BCs

$$\overline{v}^i = v_{\square}^i \text{ on } \partial\Omega_{\square}, \tag{S169}$$

$$n^{n-1/2,i}\Pi^{n-1/2,1}{}_i(V, W, \sigma^*) = 0 \text{ on } \partial\Omega_{\square}, \tag{S170}$$

$$\overline{w} = 0 \text{ on } \partial\Omega, \tag{S171}$$

$$n_i^{n-1/2}\overline{v}^i = 0 \text{ on } \partial\Omega_{\square} \cup \partial\Omega_{\circ}. \tag{S172}$$

   Here, we obtained Eqs. (S167) and (S168) from Eqs. (S150) and (S151) by replacing the velocity fields with the approximated ones or with $V$ and $W$, and similarly for Eqs. (S169) to (S172) and Eqs. (S153) to (S160).

2. **Pressure correction.**

   Subtracting Eqs. (S150) and (S167) we obtain

$$\rho\frac{v^{n,i} - \overline{v}^i}{\Delta t} = -\nabla^{n-1/2,i}\phi + O(\Delta t). \tag{S173}$$

   Taking the covariant derivative of Eq. (S173) and neglecting $O(\Delta t)$, we obtain

$$\begin{aligned}\nabla_i^{n-1/2}\nabla^{n-1/2,i}\phi &= -\frac{\rho}{\Delta t}\left(\nabla_i^{n-1/2}v^{n,i} - \nabla_i^{n-1/2}\overline{v}^i\right) \\ &= -\frac{\rho}{\Delta t}\left(2\mu^{n-1/2}w^n - \nabla_i^{n-1/2}\overline{v}^i\right),\end{aligned} \tag{S174}$$

   where in the second line we used Eq. (S149).

   We will now work out the BCs for Eq. (S174). First, Eqs. (S131) and (S157) imply the Dirichlet BC (S134). Second, by combining Eq. (S173) with Eqs. (S153), (S156), (S169) and (S172) we obtain the Neumann BC

$$n^{n-1/2,i}\nabla_i^{n-1/2}\phi = 0 \text{ on } \partial\Omega_{\square} \cup \partial\Omega_{\circ}. \tag{S175}$$

   Overall, Eqs. (S134), (S174) and (S175) constitute a Poisson-like BVP which determines $\phi$.

3. **Velocities.**

   Subtracting Eqs. (S151) and (S168) we obtain

$$\frac{\rho}{\Delta t}(w^n - \overline{w}) = O(\Delta t), \tag{S176}$$

   which implies

$$w^n = \overline{w} + O(\Delta t^2) \tag{S177}$$

Neglecting $O(\Delta t)$ in Eqs. (S173) and (S177), we obtain the relations

$$\rho \frac{v^{n,i} - \overline{v}^i}{\Delta t} = - \nabla^{n-1/2,i} \phi, \tag{S178}$$

$$w^n = \overline{w}, \tag{S179}$$

which determine $v^n$ and $w^n$, respectively, in terms of $\overline{v}$ and $\overline{w}$.

4. **Manifold.** From Eqs. (14) and (15) we obtain

$$\omega_i^{n-1/2} = \nabla_i^{n-1/2} z^{n-1/2}, \tag{S180}$$

$$\mu^{n-1/2} = H(\omega^{n-1/2}). \tag{S181}$$

We solve Eqs. (S152), (S180) and (S181) with BCs (S158) to (S160), for $z^{n-1/2}$, $\omega^{n-1/2}$ and $\mu^{n-1/2}$.

We will now discuss the variational formulation of the BVPs in Cases 1 to 4, proceeding along the lines of Section S3.2.1. We will first present the VPs, and then specify their BCs.

1. **Approximated velocities.**

We multiply Eq. (S167) by $\sqrt{|g^{n-1/2}|}\nu_{\overline{v}i}$ integrate, and obtain

$$\begin{aligned}
&\left\langle \rho \left[ \frac{\overline{v}^i - v^{n-1,i}}{\Delta t} + \left( \frac{3}{2} v^{n-1,j} - \frac{1}{2} v^{n-2,j} \right) \nabla_j^{n-1/2} V^i - 2 V^j W b^{n-1/2,i}{}_j \right] \nu_{\overline{v}i} \right\rangle_\Omega^{n-1/2} - \\
&- \frac{\rho}{2} \left[ - \left\langle W^2 \nabla_i^{n-1/2} \nu_{\overline{v}}{}^i \right\rangle_\Omega^{n-1/2} + \left\langle W^2 n_i^{n-1/2} \nu_{\overline{v}}{}^i \right\rangle_{\partial\Omega}^{n-1/2} \right] + \left\langle \sigma^* \nabla_i^{n-1/2} \nu_{\overline{v}}{}^i \right\rangle_\Omega^{n-1/2} - \left\langle \sigma^* n_i^{n-1/2} \nu_{\overline{v}}{}^i \right\rangle_{\partial\Omega}^{n-1/2} - \\
&- 2\eta \Big[ - \left\langle d^{ij}(V, W, \omega^{n-1/2}) \nabla_i^{n-1/2} \nu_{\overline{v}j} \right\rangle_\Omega^{n-1/2} + \left\langle n_i^{n-1/2} d^{ij}(V, W, \omega^{n-1/2}) \nu_{\overline{v}j} \right\rangle_{\partial\Omega_\square \cup \partial\Omega_\bigcirc}^{n-1/2} + \\
&+ \left\langle n_i^{n-1/2} d^{i2}(V, W, \omega^{n-1/2}) \nu_{\overline{v}2} \right\rangle_{\partial\Omega_{\square}}^{n-1/2} \Big] = 0,
\end{aligned} \tag{S182}$$

where we used Eqs. (S18) and (S19), and we have set

$$\langle \cdot \rangle_\Omega^{n-1/2} \equiv \int_\Omega dx^1 dx^2 \sqrt{|g^{n-1/2}|} \, \cdot, \tag{S183}$$

$$\langle \cdot \rangle_{\partial\Omega}^{n-1/2} \equiv \int_{\partial\Omega} ds \sqrt{|h^{n-1/2}|} \, \cdot, \tag{S184}$$

and here and in what follows indices are raised an lowered with the metric $g^{n-1/2}$. In the last line of Eq. (S182), we imposed Eq. (S170) as a natural BC by using Eqs. (S23), (S124) and (S157).

Proceeding along the same lines, we multiply Eq. (S168) by $\sqrt{|g^{n-1/2}|}\nu_{\overline{w}}$ integrate, and obtain

$$\left\langle \rho \left( \frac{w^n - \overline{w}}{\Delta t} + V^i V^j b_{ij}^{n-1/2} \right) \nu_{\overline{w}} \right\rangle_\Omega^{n-1/2} +$$

$$\rho \left\{ - \left\langle W \nabla_i^{n-1/2} \left[ \left( \frac{3}{2} v^{n-1,i} - \frac{1}{2} v^{n-2,i} \right) \nu_{\overline{w}} \right] \right\rangle_\Omega^{n-1/2} + \left\langle n_i^{n-1/2} W \left( \frac{3}{2} v^{n-1,i} - \frac{1}{2} v^{n-2,i} \right) \nu_{\overline{w}} \right\rangle_{\partial\Omega}^{n-1/2} \right\} +$$

$$+2\kappa \left\{ \left\langle - \left( \nabla^{n-1/2,i} \mu^{n-1/2} \right) \nabla_i^{n-1/2} \nu_{\overline{w}} + 2\mu^{n-1/2} \left[ (\mu^{n-1/2})^2 - K^{n-1/2} \right] \nu_{\overline{w}} \right\rangle_\Omega^{n-1/2} + \right.$$

$$\left. + \left\langle n_i^{n-1/2} \left( \nabla^{n-1/2,i} \mu^{n-1/2} \right) \nu_{\overline{w}} \right\rangle_{\partial\Omega}^{n-1/2} \right\} -$$

$$-2 \left\langle \left[ \sigma^* \mu^{n-1/2} + \mathfrak{f}_\eta (V, W, \omega^{n-1/2}) \right] \nu_{\overline{w}} \right\rangle_\Omega^{n-1/2} = 0, \tag{S185}$$

where we used Eqs. (S18) and (S19).

2. **Pressure correction.**
From Eqs. (S18) and (S174), we obtain

$$\left\langle (\nabla^{n-1/2,i} \phi) \nabla_i^{n-1/2} \nu_\phi \right\rangle_\Omega^{n-1/2} + \frac{\rho}{\Delta t} \left\langle \left( \nabla_i^{n-1/2} \overline{v}^i - 2\mu^{n-1/2} \overline{w} \right) \nu_\phi \right\rangle_\Omega^{n-1/2} - \\ - \left\langle n^{n-1/2,i} \left( \nabla_i^{n-1/2} \phi \right) \nu_\phi \right\rangle_{\partial\Omega}^{n-1/2} = 0, \tag{S186}$$

where we imposed Eq. (S175) as a natural BC.

3. **Velocities.**
Neglecting $O(\Delta t)$, Eqs. (S178) and (S179) imply

$$\left\langle \left[ \frac{\rho}{\Delta t} (v^{n,i} - \overline{v}^i) + \nabla^{n-1/2,i} \phi \right] \nu_{v^n i} \right\rangle_\Omega^{n-1/2} = 0, \tag{S187}$$

$$\langle (w^n - \overline{w}) \nu_{w^n} \rangle_\Omega^{n-1/2} = 0. \tag{S188}$$

4. **Manifold.**
Equations (S152), (S180) and (S181) imply

$$\left\langle \omega_i^{n-1/2} \nu_{z^{n-1/2}}{}^i + \left( \nabla_i^{n-1/2} \nu_{\omega^{n-1/2}}{}^i \right) z^{n-1/2} \right\rangle_\Omega^{n-1/2} - \left\langle z^{n-1/2} n_i^{n-1/2} \nu_{\omega^{n-1/2}}{}^i \right\rangle_{\partial\Omega}^{n-1/2} = 0, \tag{S189}$$

$$\left\langle \left[ \mu^{n-1/2} - H(\omega^{n-1/2}) \right] \nu_{\mu^{n-1/2}} \right\rangle_\Omega^{n-1/2} = 0, \tag{S190}$$

$$\left\langle \left[ \frac{z^{n-1/2} - z^{n-3/2}}{\Delta t} - w^{n-1} \left( \hat{N}^{n-1/2,3} - \hat{N}^{n-1/2,i} \omega_i^{n-1/2} \right) \right] \nu_{z^{n-1/2}} \right\rangle_\Omega^{n-1/2} = 0. \tag{S191}$$

Unlike the case of a fixed $\mathscr{M}$, Section S3.2.1, here the steps of the splitting scheme cannot be solved separately, because they are coupled through the manifold shape. As a result, the VPs (S182) and (S185) to (S191) will be solved as a mixed VP [15, 14] for the unknowns $\overline{v}$, $\overline{w}$ $v^n$, $w^n$, $\phi$, $z^{n-1/2}$, $\omega^{n-1/2}$ and $\mu^{n-1/2}$.

In addition to the natural BCs (S170) and (S175), we impose Eqs. (S134), (S158) to (S160), (S169) and (S171) as Dirichlet BCs. Finally, we enforce Eq. (S172) and the relation between $\mu^{n-1/2}$ and $H$ on $\partial\Omega$, i.e.,

$$\mu^{n-1/2} = H(\omega^{n-1/2}) \text{ on } \partial\Omega. \tag{S192}$$

with the penalty method, by adding the functional

$$G_\mu \equiv \frac{\alpha}{l} \left\langle [\mu^{n-1/2} - H(\omega^{n-1/2})] \nu_{\mu^{n-1/2}} \right\rangle_{\partial\Omega}, \tag{S193}$$

cf. Eq. (S33).

Finally, we iterate in time by updating the fields along the lines of Section S3.2.1. This dynamics is solved in the `dynamics` module as `variational_problem_bc_square_a`, see Fig. 5.

## S3.3 Exact solutions

### S3.3.1 Radially symmetric steady state with no flows

In this Section, we will show how to obtain a numerically exact solution for the steady state in the absence of flows in the radially symmetric case discusses in Section 3.1.1.

We will use the radial coordinates $r$, $\theta$ discussed in Section S1.7, for which the quantities in Section S1 read

$$\boldsymbol{X} = (r\cos\theta, r\sin\theta, z(r)), \tag{S194}$$
$$\mathbf{e}_1 = (\cos\theta, \sin\theta, \partial_r z), \tag{S195}$$
$$\mathbf{e}_2 = (-r\sin\theta, r\cos\theta, 0), \tag{S196}$$
$$g_{ij} = \begin{pmatrix} 1+\omega_r^2 & 0 \\ 0 & r^2 \end{pmatrix}, \tag{S197}$$
$$g^{ij} = \frac{1}{|g|}\begin{pmatrix} r^2 & 0 \\ 0 & 1+\omega_r^2 \end{pmatrix}, \tag{S198}$$
$$|g| = r^2(1+\omega_r^2), \tag{S199}$$
$$b_{ij} = \frac{r}{\sqrt{|g|}}\begin{pmatrix} \partial_r\omega_r & 0 \\ 0 & r\omega_r \end{pmatrix}, \tag{S200}$$

where

$$\omega_r = \partial_r z. \tag{S201}$$

We will now work out the terms in the force-balance equation (13). First, by using Eqs. (S10), (S197) and (S199), we obtain

$$\nabla_{\mathrm{LB}} H = \frac{1}{\sqrt{|g|}}\partial_r\left(\frac{r^2\partial_r H}{\sqrt{|g|}}\right). \tag{S202}$$

Second, by using Eqs. (S6), (S7), (S199) and (S200) we obtain the following expressions for the mean and Gaussian curvature:

$$H(r) = \frac{1}{2|g|^{3/2}}\left(\omega_r|g| + r^3\partial_r\omega_r\right), \tag{S203}$$
$$K(r) = -\frac{1}{2r}\partial_r\left(\frac{r^2}{|g|}\right). \tag{S204}$$

Combining Eqs. (13) and (S202) to (S204), we obtain a fourth-order ordinary differential equation (ODE) for $z$ which can be solved in a numerically exact way, see `check_with_analytical_solution_bc_ring`. The solution is shown in panels C to E of Fig. S1.

### S3.3.2 Radially symmetric steady state with flows

In this Section, we will show how to obtain a numerically exact solution for the steady state with flows in the radially symmetric case discusses in Section 3.1.2.

Given Eqs. (S194) to (S204), which still hold in the presence of flows, in what follows we will discuss the geometrical in quantities which involve the velocity field. First, we observe that radial symmetry implies that

$$v^\theta = 0. \tag{S205}$$

The only non-vanishing Christoffel symbols (S9) are [1]

$$\Gamma^r_{rr} = \frac{\omega_r \partial_r \omega_r}{|g|}, \tag{S206}$$

$$\Gamma^r_{\theta\theta} = -\frac{r}{|g|}, \tag{S207}$$

$$\Gamma^\theta_{r\theta} = \Gamma^\theta_{\theta r} = \frac{1}{r}. \tag{S208}$$

The only non-vanishing components of $\nabla_i v^j$ are

$$\nabla_r v^r = \nabla^r v_r = \partial_r v^r + v^r \Gamma^r_{rr}, \tag{S209}$$

$$\nabla_\theta v^\theta = \nabla^\theta v_\theta = v^r \Gamma^\theta_{\theta r}, \tag{S210}$$

where we used Eqs. (S8) and (S205).

We will now work out the terms in Eqs. (18) to (20). First, Eq. (18) can be rewritten as

$$\begin{aligned} \nabla_i v^i =& \partial_r v^r + v^r \left(\Gamma^r_{rr} + \Gamma^\theta_{r\theta}\right) \\ =& \partial_r v^r + v^r \left(\frac{\omega_r \partial_r \omega_r}{1+\omega_r^2} + \frac{1}{r}\right) \\ =& \partial_r v^r + v^r \left[\frac{1}{2}\partial_r \log(1+\omega_r^2) + \frac{1}{r}\right], \end{aligned} \tag{S211}$$

where we used Eqs. (S8), (S206) and (S208). We rewrite Eq. (S211) as

$$\partial_r \left[\log(r v^r) + \frac{1}{2}\log\left(1+\omega_r^2\right)\right] = 0, \tag{S212}$$

and by integrating we obtain

$$v^r = \frac{C}{r\sqrt{1+\omega_r^2}}, \tag{S213}$$

where $C$ is an integration constant. Physically, Eq. (S213) constitutes the relation between the radial fluid velocity and manifold shape which needs to hold for the fluid mass to be conserved according to Eq. (18).

In order simplify the other equations we observe that, given that we are at steady state, we must have

$$w = 0 \tag{S214}$$

everywhere. The viscous term in the right-hand side (RHS) of Eq. (19) thus reads

$$\begin{aligned} -\nabla_{\mathrm{LB}} v^i - 2\left(b^{ij} - 2\,\mu\, g^{ij}\nabla_j w\right) + 2K v^i =& \nabla^j \nabla_j v^i + \nabla^j \nabla^i v_j \\ =& 2\left[\partial_r \nabla_r v^r + (\nabla_r v^r)\Gamma^\theta_{\theta r} - (\nabla_\theta v^\theta)\Gamma^\theta_{\theta r}\right] \end{aligned} \tag{S215}$$

where we used Eqs. (S8), (S22), (S25) and (S214). The first term in the LHS of Eq. (20) can be rewritten as

$$v^i v^j b_{ji} = (v^r)^2 b_{rr}, \tag{S216}$$

where we used Eq. (S200). Finally, we rewrite the viscous term in the RHS of Eq. (20) as

$$(\nabla^i v^j) b_{ij} = g^{rr}(\nabla_r v^r) b_{rr} + g^{\theta\theta}(\nabla_\theta v^\theta) b_{\theta\theta}, \tag{S217}$$

where we used Eq. (S200).

Combining Eqs. (19), (20) and (S214) to (S217), we obtain the following system of ODEs:

$$\rho v^r \nabla_r v^r - g^{rr}\partial_r \sigma - 2\eta g^{rr}\left[\partial_r \nabla_r v^r + (\nabla_r v^r)\Gamma^\theta_{\theta r} - (\nabla_\theta v^\theta)\Gamma^\theta_{\theta r}\right] = 0, \tag{S218}$$

$$\begin{aligned} \rho (v^r)^2 b_{rr} + 2\kappa \left[\frac{1}{\sqrt{|g|}}\partial_r\left(\frac{r^2 \partial_r H}{\sqrt{|g|}}\right) + 2H(H^2-K)\right] - 2\sigma H - \\ 2\eta\left[g^{rr}(\nabla_r v^r) b_{rr} + g^{\theta\theta}(\nabla_\theta v^\theta) b_{\theta\theta}\right] = 0. \end{aligned} \tag{S219}$$

Since the radial velocity $v^r$ depends on $z$ through Eq. (S213), Eqs. (S217) and (S218) constitute a system of ODEs for the unknowns $\sigma$ and $z$. The explicit expressions for the quantities which enter in Eqs. (S217) and (S218) can be obtained by means of Eqs. (S206) to (S210).

This ODE system is solved in a numerically exact way in `check_with_analytical_solution_bc_ring_1` and `check_with_analytical_solution_bc_ring_2`; the solution is shown in panels E to I of Figs. S2 and S3.

#### S3.3.3 Channel flow on a fixed manifold

In what follows, we will solve the steady state of Eqs. (23) and (24), which describe the channel flow on a fixed manifold, for a problem invariant with respect to translations along the $x^1$ axis. The result will be an exact solution obtained by quadratures.

The surface parametrization (S1), tangent vectors (S2), metric tensor (S4) read

$$\boldsymbol{X}(x^1, x^2) =(x^1, x^2, z(x^2)), \tag{S220}$$

$$\mathbf{e}_1 =(1, 0, 0), \tag{S221}$$

$$\mathbf{e}_2 =(0, 1, \omega_2), \tag{S222}$$

$$g_{ij} = \begin{pmatrix} 1 & 0 \\ 0 & 1+\omega_2^2 \end{pmatrix}, \tag{S223}$$

$$g^{ij} = \begin{pmatrix} 1 & 0 \\ 0 & 1/|g| \end{pmatrix}, \tag{S224}$$

$$|g| =1 + \omega_2^2, \tag{S225}$$

At steady state, symmetry implies [10]

$$v^2 =0, \tag{S226}$$

$$\partial_1 v^1 =0, \tag{S227}$$

$$\tag{S228}$$

Let us work out the quantities which enter in (23) and (24). By using Eqs. (S8), (S9), (S223), (S226) and (S227) we have

$$\nabla_1 v^1 = \nabla_2 v^2 =0, \tag{S229}$$

$$v^i \nabla_i v^1 =0. \tag{S230}$$

The Laplace-Beltrami ds operator applied to the velocity reads

$$\begin{aligned}
\nabla_{\text{LB}} v^1 &= -\sqrt{|g|} g^{11} g^{22} \epsilon_{21} \partial_2 \left[ \sqrt{|g|} g^{22} g^{11} \epsilon_{21} \partial_2 \left( g_{11} v^1 \right) \right] \\
&= -\frac{1}{\sqrt{|g|}} \partial_2 \left( \frac{v^2}{\sqrt{|g|}} \right), \\
\nabla_{\text{LB}} v^2 &= -\sqrt{|g|} g^{22} g^{11} \epsilon_{12} \partial_1 \left[ \sqrt{|g|} g^{mn} g^{op} \epsilon_{mo} \partial_n \left( g_{pq} v^q \right) \right] \\
&= 0,
\end{aligned} \tag{S231}$$

where we used Eqs. (S11), (S220), (S223) and (S226) to (S227). The covariant derivatives of the surface tension read

$$\nabla^1 \sigma =\partial_1 \sigma, \tag{S232}$$

$$\nabla^2 \sigma =\frac{1}{\sqrt{|g|}} \partial_2 \sigma, \tag{S233}$$

where we used Eqs. (S8) and (S224).

Equation (S229) implies that the continuity equation (23) is identically satisfied. On the other hand, from Eqs. (S231) to (S233), we obtain the two components of the NS equations (24):

$$\partial_1 \sigma + \eta \frac{1}{\sqrt{|g|}} \partial_2 \left( \frac{\partial_2 v}{\sqrt{|g|}} \right) = 0, \tag{S234}$$

$$\partial_2 \sigma = 0. \tag{S235}$$

Equation (S235) implies that $\sigma$ depends on $x^1$ only: By substituting this result in Eq. (S234), we have

$$\partial_1 \sigma = C = \eta \frac{1}{\sqrt{|g|}} \partial_2 \left( \frac{\partial_2 v}{\sqrt{|g|}} \right), \tag{S236}$$

where $C$ is independent of $\boldsymbol{x}$. We solve Eq. (S236) by quadrature by imposing the BC (S109), and obtain

$$v^1(x^2) = \frac{C}{\eta} \int_0^{x^2} \mathrm{d}v \sqrt{|g(v)|} \left[ \int_0^v \mathrm{d}u \sqrt{|g(u)|} - C \right], \tag{S237}$$

where we wrote explicitly the spatial dependence of $g$ on the spatial coordinate. We observe that Eq. (S237) is the analog of the solution for channel flow on a flat manifold [10], with the linear measure $dx^2$ replaced by $\sqrt{|g|}dx^2$.

The solution (S237) with model parameters (25) is depicted in Fig. S5.

# Acronyms

**BC** boundary condition, 4–6, 8–11, 15–24, 28

**BVP** boundary-value problem, 5, 6, 10, 15, 16, 22, 23

**CN** Crank Nicolson, 15

**FE** finite element, 30

**FEniCS** finite element computational software, 29

**IPCS** incremental pressure correction scheme, 15, 22

**LHS** left-hand side, 8, 26

**NS** Navier-Stokes, 15, 28

**ODE** ordinary differential equation, 25–27

**PDE** partial differential equation, 5

**RHS** right-hand side, 26

**TMP** trans-membrane protein, 7, 12–14

**VP** variational problem, 3–6, 9–11, 17, 18, 23, 24

# Glossary

$H$ mean curvature [3]. 7, 28, 29

$K$ Gaussian curvature [3]. 28

$\mathbf{c}$ center of the circular obstacle in a mesh. 28

$\boldsymbol{x}$ coordinates on $\mathscr{M}$. 28

$\epsilon_{ij}$ Levi-Civita antisymmetric symbol [1]. 2, 28

$\kappa$ bending rigidity [22]. 28

$\mu$ auxiliary variable which equals the mean curvature $H$, see Eq. (15). It is a scalar on $\mathscr{M}$. 4, 12, 28

$\nabla$ covariant derivative [1]. 28

$\nabla_{\mathbf{LB}}$ Laplace-Beltrami operator [6]. 28

$\hat{N}$ unit vector in the three-dimensional Euclidean space, normal to $\mathscr{M}$, see Fig. 1. 1, 4, 28

$\omega$ gradient of $z$, it is a one-form on $\mathscr{M}$. 4, 28, 29, 30

$\omega_r$ radial component of $\omega$ in polar coordinates. 12, 28

$\sigma$ surface tension [22], it is a scalar on $\mathscr{M}$. 12, 28

$\hat{x}$ radial direction: $\hat{x}^i = \frac{x^i}{|\mathbf{x}|}$. 28

$b$ second fundamental form [1]. 1, 28

$g$ metric tensor [1]. 1, 3, 28

$h$ pull-back of the metric $g$ on a curve $\gamma$ in $\mathscr{M}$ [1, 7]. 2, 3, 4, 28

$n$ unit vector in the tangent bundle of $\mathscr{M}$ and normal to a curve in $\mathscr{M}$, see Fig. 1. 3, 5, 6, 8, 28

$r$ radius of circular obstacle in a mesh. 28

$v$ tangential velocity, it is a vector field the tangent bundle of $\mathscr{M}$. 12, 19, 28

$w$ normal velocity, it is a scalar on $\mathscr{M}$. 28

$z$ fluid shape profile, it is a scalar on $\mathscr{M}$. 4, 7, 12, 19, 28, 29

**finite element computational software (FEniCS)** finite element computational software [14], on which irene is built.. 28

$L$ length of a rectangle which defines $\omega$. 19, 28

$l$ mesh cell size: the smallest cell diameter, across all cells in the mesh. 4, 28

$\eta$ two-dimensional viscosity [10]. 28

$\gamma$ a curve in $\mathscr{M}$. 2, 28, 29

$\mathscr{M}$ differential manifold [1]. 1, 2, 3, 4, 6, 24, 28, 29

$\mathfrak{n}$ vector normal to a curve $\gamma$ in $\mathscr{M}$; this vector belongs to the tangent bundle of $\mathscr{M}$ [1]. 2, 4, 28

$\Omega$ subset of $\mathbb{R}^2$ over which the coordinates of $\mathscr{M}$ are defined [16]. 3, 28, 29, 30

$\partial\Omega$ boundary of $\Omega$, see Fig. 1 and Eq. (7). 3, 4, 28

$\partial\Omega_{\underline{\square}}$ boundary of $\Omega$ located at the bottom edge of the rectangle. 2, 28

$\partial\Omega_{\circ}$ circular boundary of $\Omega$. 3, 28

$\partial\Omega_{\odot}$ inner circular boundary of $\Omega$. 5, 28, 30

$\partial\Omega_{\bigcirc}$ same as $\partial\Omega_{\odot}$, for the outer circular boundary. 5, 28

$\partial\Omega_{\llcorner}$ boundary of $\Omega$ located at the left edge of the rectangle. 28, 30

$\partial\Omega_{\sqsubset}$ $\partial\Omega_{\llcorner} \cup \partial\Omega_{=}$. 28

$\partial\Omega_{\lrcorner}$ same as $\partial\Omega_{\llcorner}$, for the right edge of the rectangle. 10, 28

$\partial\Omega_{\square}$ rectangular boundary of $\Omega$, see Eq. (6). 28

$\partial\Omega_{-}$ boundary of $\Omega$ located at the top edge of the rectangle. 28

$\partial\Omega_{=}$ same as $\partial\Omega_{\llcorner}$, for the top and bottom edges of the rectangle, see Eq. (5). 28, 30

$v$ test function in finite element (FE) methods [15]. In irene, it is denoted by the suffix of its related function, e.g., the test function related to $z$ is $v_z$. 28

$\rho$ density [10]. 28

$h$ height of a rectangle which defines $\omega$. 19, 28

**element** an atomic part of a mesh [15, 23]. 28

# References


[1] S. Marchiafava. *Appunti Di Geometria Differenziale*, volume I, II, III. Edizioni Nuova Cultura, 2005.

[2] T. Frankel. *The Geometry of Physics: An Introduction*. Cambridge University Press, 3 edition, Nov. 2011.

[3] M. Deserno. Notes on Differential Geometry. https://www.cmu.edu/biolphys/deserno/pdf/diff_geom.pdf, 2004.

[4] P. Howell, G. Zoyreff, and J. Ockendon. *Applied Solid Mechanics*. Cambridge University Press, 2008.

[5] J. E. Marsden and T. J. R. Hughes. *Mathematical Foundations of Elasticity*. Dover, New York, 1994.

[6] M. Arroyo and A. DeSimone. Relaxation dynamics of fluid membranes. *Phys. Rev. E*, 79(3):031915, Mar. 2009.

[7] H. Reall. General Relativity. https://www.damtp.cam.ac.uk/user/hsr1000/teaching.html.

[8] C.-C. Hsiung. *A First Course in Differential Geometry*. John Wiley & Sons, New York, USA, 1981.

[9] S. C. Al-Izzi, P. Sens, and M. S. Turner. Shear-Driven Instabilities of Membrane Tubes and Dynamin-Induced Scission. *Phys. Rev. Lett.*, 125(1):018101, July 2020.

[10] L. D. Landau and E. M. Lifschitz. *Fluid Mechanics*. Pergamon, 1987.

[11] I. Babuska. The Finite Element Method with Penalty. *Mathematics of Computation*, 27(122):221, Apr. 1973.

[12] V. J. Nitsche. Über ein Yariationsprinzip zur Liisung yon Dirichlet-Problemen bei Verwendung yon Teilräumen, die keinen Randbedingungen unterworfen sind. *Abhandlungen aus dem Mathematischen Seminar der Universität Hamburg*, 36:9–15, 1971.

[13] A. Bansal, N. A. Barnafi, and D. N. Pandey. Nitsche method for Navier–Stokes equations with slip boundary conditions: Convergence analysis and VMS-LES stabilization. *ESAIM: M2AN*, 58(5):2079–2115, Sept. 2024.

[14] A. Logg, K.-A. Mardal, and G. Wells, editors. *Automated Solution of Differential Equations by the Finite Element Method: The FEniCS Book*, volume 84 of *Lecture Notes in Computational Science and Engineering*. Springer Berlin Heidelberg, Berlin, Heidelberg, 2012.

[15] O. C. Zienkiewicz, R. L. Taylor, and J. Z. Zhu. *The Finite Element Method: Its Basis and Fundamentals*. Elsevier, Butterworth-Heinemann, Amsterdam, 7th edition edition, 2013.

[16] L. C. Evans. *Partial Differential Equations*. Graduate Studies in Mathematics. American Mathematical Society, 2010.

[17] J. Crank and P. Nicolson. A practical method for numerical evaluation of solutions of partial differential equations of the heat-conduction type. *Math. Proc. Camb. Phil. Soc.*, 43(1):50–67, Jan. 1947.

[18] A. J. Chorin. Numerical solution of the Navier-Stokes equations. *Math. Comp.*, 22(104):745–762, 1968.

[19] R. Témam. Sur l'approximation de la solution des équations de Navier-Stokes par la méthode des pas fractionnaires (I). *Arch. Rational Mech. Anal.*, 32:135–153, 1968.

[20] K. Goda. A multistep technique with implicit difference schemes for calculating two- or three-dimensional cavity flows. *Journal of Computational Physics*, 30(1):76–95, Jan. 1979.

[21] H. Blum, J. Harig., S. Müller, S. Schreiber, and S. Turek. FEAT2D, Finite Element Analysis Tools User Manual, 1995.

[22] I. Derényi, F. Jülicher, and J. Prost. Formation and Interaction of Membrane Tubes. *Phys. Rev. Lett.*, 88(23):238101, May 2002.

[23] Y. Liu. Lecture Notes: An Introduction to the Finite Element Method, 1997.
